# Supplementary material for: Optimized Runge-Kutta Methods with Automatic Step Size Control for Compressible Computational Fluid Dynamics
Source: arXiv:2104.06836 source file (2021-07-24)
Supplement: Supplementary file 1 [file supplement.pdf]

# Optimized Runge-Kutta Methods with Automatic Step Size Control for Compressible Computational Fluid Dynamics: Supplementary Material

Hendrik Ranocha    Lisandro Dalcin    Matteo Parsani
David I. Ketcheson

April 14, 2021

This document includes supplementary material for the paper *Optimized Runge-Kutta Methods with Automatic Step Size Control for Compressible Computational Fluid Dynamics*. This includes additional properties of the Runge-Kutta pairs discussed in the paper and results of additional numerical experiments.

## 1 Properties of the Runge-Kutta pairs

Table 1 gives the values of certain measures used to predict the accuracy and efficiency of Runge-Kutta pairs, for each of the pairs discussed in the paper. For the definitions of these quantities, see [37].

Table 1: Characteristics of the Runge-Kutta methods. $\iota_r$ is the length of the real stability interval. The remaining quantities are defined in [37].

| Scheme | $A^{q+1}$ | $A^{q+2}$ | $\widehat{A}^{\widehat{q}+1}$ | $B^{\widehat{q}+2}$ | $C^{\widehat{q}+2}$ | $D$ | $E^{\widehat{q}+2}$ | $\iota_r$ |
|---|---|---|---|---|---|---|---|---|
| | $A_\infty^{q+1}$ | $A_\infty^{q+2}$ | $\widehat{A}_\infty^{\widehat{q}+1}$ | $B_\infty^{\widehat{q}+2}$ | $C_\infty^{\widehat{q}+2}$ | | $E_\infty^{\widehat{q}+2}$ | $\iota_r/s$ |
| BS3(2)3$_F$ | 4.18e-02 | 4.40e-02 | 2.95e-02 | 1.35e+00 | 1.38e+00 | 1.00 | 1.42e+00 | 2.51 |
| | 4.17e-02 | 3.33e-02 | 2.08e-02 | 1.50e+00 | 1.50e+00 | | 2.00e+00 | 0.84 |
| BS5(4)7$_F$ | 2.22e-05 | 2.13e-04 | 1.06e-04 | 1.04e+00 | 1.04e+00 | 1.16 | 2.09e-01 | 3.99 |
| | 1.27e-05 | 9.09e-05 | 7.71e-05 | 6.40e-01 | 7.63e-01 | | 1.65e-01 | 0.57 |
| DP5(4)6$_F$ | 3.99e-04 | 3.96e-03 | 1.18e-03 | 1.54e+00 | 1.67e+00 | 9.82 | 3.37e-01 | 3.31 |
| | 2.78e-04 | 3.73e-03 | 8.08e-04 | 1.24e+00 | 1.33e+00 | | 3.44e-01 | 0.55 |
| SSP3(2)3[3S*$_+$] | 7.22e-02 | 5.65e-02 | 6.98e-02 | 1.23e+00 | 6.71e-01 | 1.00 | 1.03e+00 | 2.51 |
| | 4.17e-02 | 3.33e-02 | 6.24e-02 | 1.17e+00 | 5.00e-01 | | 6.68e-01 | 0.84 |
| SSP3(2)4[3S*$_+$] | 3.61e-02 | 3.02e-02 | 4.66e-02 | 9.75e-01 | 5.92e-01 | 1.00 | 7.75e-01 | 5.15 |
| | 2.08e-02 | 2.29e-02 | 4.17e-02 | 7.50e-01 | 5.00e-01 | | 5.00e-01 | 1.29 |
| KCL3(2)4[2R$_+$]C | 1.12e-02 | 1.31e-02 | 4.05e-02 | 6.27e-01 | 5.42e-01 | 2.98 | 2.75e-01 | 2.79 |
| | 1.11e-02 | 8.33e-03 | 3.33e-02 | 6.10e-01 | 5.96e-01 | | 3.32e-01 | 0.70 |
| KCL4(3)5[2R$_+$]C | 5.12e-03 | 7.45e-03 | 8.83e-03 | 1.41e+00 | 9.64e-01 | 0.85 | 5.80e-01 | 4.82 |
| | 3.48e-03 | 2.84e-03 | 5.95e-03 | 1.03e+00 | 8.71e-01 | | 5.84e-01 | 0.96 |
| KCL4(3)5[3R$_+$]C | 3.86e-03 | 4.72e-03 | 6.49e-03 | 1.15e+00 | 8.08e-01 | 1.00 | 5.94e-01 | 4.66 |
| | 3.33e-03 | 2.55e-03 | 5.95e-03 | 7.03e-01 | 5.92e-01 | | 5.60e-01 | 0.93 |
| KCL5(4)9[2R$_+$]S | 1.01e-03 | 1.50e-03 | 2.12e-03 | 1.62e+00 | 1.40e+00 | 1.01 | 4.78e-01 | 6.31 |
| | 4.87e-04 | 6.29e-04 | 1.29e-03 | 1.37e+00 | 1.31e+00 | | 3.79e-01 | 0.70 |
| RK3(2)5[3S*$_+$] | 9.93e-03 | 1.15e-02 | 3.09e-03 | 3.68e+00 | 9.60e-01 | 0.89 | 3.22e+00 | 4.93 |
| | 9.93e-03 | 8.01e-03 | 2.78e-03 | 3.96e+00 | 8.75e-01 | | 3.57e+00 | 0.99 |
| RK3(2)5$_F$[3S*$_+$] | 9.93e-03 | 1.15e-02 | 6.43e-03 | 1.78e+00 | 1.67e+00 | 1.00 | 1.55e+00 | 4.93 |
| | 9.93e-03 | 8.01e-03 | 5.90e-03 | 1.49e+00 | 1.49e+00 | | 1.68e+00 | 0.99 |
| RK4(3)9[3S*$_+$] | 5.06e-04 | 1.93e-03 | 3.89e-03 | 1.04e+00 | 1.01e+00 | 1.97 | 1.30e-01 | 9.47 |
| | 5.06e-04 | 1.01e-03 | 3.36e-03 | 6.92e-01 | 6.92e-01 | | 1.51e-01 | 1.05 |
| RK4(3)9$_F$[3S*$_+$] | 5.06e-04 | 1.93e-03 | 2.02e-03 | 1.36e+00 | 1.34e+00 | 1.97 | 2.51e-01 | 9.47 |
| | 5.06e-04 | 1.01e-03 | 1.85e-03 | 1.25e+00 | 1.25e+00 | | 2.73e-01 | 1.05 |
| RK5(4)10[3S*$_+$] | 5.10e-05 | 1.86e-04 | 1.82e-04 | 8.17e-01 | 7.02e-01 | 2.19 | 2.80e-01 | 8.23 |
| | 2.54e-05 | 1.01e-04 | 1.07e-04 | 8.30e-01 | 6.53e-01 | | 2.36e-01 | 0.82 |
| RK5(4)10$_F$[3S*$_+$] | 5.10e-05 | 1.86e-04 | 2.42e-04 | 1.80e+00 | 1.75e+00 | 2.19 | 2.11e-01 | 8.23 |
| | 2.54e-05 | 1.01e-04 | 1.48e-04 | 1.76e+00 | 1.63e+00 | | 1.72e-01 | 0.82 |

# 2 Detailed results for the inviscid test problems

Here, we provide detailed performance characteristics of the numerical methods for numerical studies described in Sections 5 and 6 of the manuscript.

## 2.1 General purpose methods

Table 2: Performance of general purpose schemes: Number of function evaluations (#FE), rejected steps (#R), and $L^2$ error of the density for the inviscid Taylor Green vortex (5.3), the isentropic vortex (5.4) , and the flow with source term (5.5) using polynomials of degree $p = 2$.

| | | | TGV (5.3) | | Isent. vortex (5.4) | | | Source term (5.5) | | |
|---|---|---|---|---|---|---|---|---|---|---|
| Scheme | $\beta$ | tol | #FE | #R | #FE | #R | Error | #FE | #R | Error |
| BS3(2)3$_F$ | $(0.60, -0.20, 0.00)$ | $10^{-1}$ | 6114 | (446) | 1685 | (153) | $5.61 \times 10^{-4}$ | 22164 | (976) | $2.99 \times 10^{-1}$ |
| | | $10^{-2}$ | 5220 | (4) | 1611 | (72) | $5.78 \times 10^{-4}$ | 20663 | (5) | $7.98 \times 10^{-3}$ |
| | | $10^{-3}$ | 5244 | (2) | 1446 | (1) | $5.76 \times 10^{-4}$ | 20646 | (5) | $1.76 \times 10^{-3}$ |
| | | $10^{-4}$ | 5256 | (2) | 1449 | (0) | $5.76 \times 10^{-4}$ | 20649 | (4) | $1.77 \times 10^{-3}$ |
| | | $10^{-5}$ | 5256 | (1) | 1476 | (0) | $5.77 \times 10^{-4}$ | 20682 | (4) | $1.77 \times 10^{-3}$ |
| | | $10^{-6}$ | 5268 | (2) | 2379 | (0) | $5.78 \times 10^{-4}$ | 20688 | (2) | $1.77 \times 10^{-3}$ |
| | | $10^{-7}$ | 5326 | (1) | 5088 | (0) | $5.78 \times 10^{-4}$ | 20940 | (2) | $1.77 \times 10^{-3}$ |
| | | $10^{-8}$ | 5659 | (24) | 10935 | (0) | $5.78 \times 10^{-4}$ | 22698 | (0) | $1.77 \times 10^{-3}$ |
| BS5(4)7$_F$ | $(0.28, -0.23, 0.00)$ | $10^{-1}$ | 8441 | (87) | 2393 | (27) | $5.78 \times 10^{-4}$ | 35538 | (312) | $4.32 \times 10^{-2}$ |
| | | $10^{-2}$ | 8548 | (75) | 2360 | (22) | $5.78 \times 10^{-4}$ | 36363 | (250) | $3.09 \times 10^{-2}$ |
| | | $10^{-3}$ | 8463 | (63) | 2342 | (17) | $5.78 \times 10^{-4}$ | 31752 | (36) | $2.49 \times 10^{-2}$ |
| | | $10^{-4}$ | 7715 | (1) | 2383 | (13) | $5.78 \times 10^{-4}$ | 30440 | (4) | $3.67 \times 10^{-3}$ |
| | | $10^{-5}$ | 7722 | (1) | 2159 | (0) | $5.78 \times 10^{-4}$ | 30356 | (2) | $1.77 \times 10^{-3}$ |
| | | $10^{-6}$ | 7731 | (0) | 2215 | (0) | $5.78 \times 10^{-4}$ | 30381 | (2) | $3.61 \times 10^{-3}$ |
| | | $10^{-7}$ | 7738 | (0) | 2383 | (0) | $5.78 \times 10^{-4}$ | 30418 | (3) | $1.77 \times 10^{-3}$ |
| | | $10^{-8}$ | 7752 | (0) | 3230 | (0) | $5.78 \times 10^{-4}$ | 30432 | (3) | $1.77 \times 10^{-3}$ |
| DP5(4)6$_F$ | $(0.70, -0.40, 0.00)$ | $10^{-1}$ | 9498 | (290) | 2677 | (99) | $5.78 \times 10^{-4}$ | 38018 | (1136) | $2.20 \times 10^{-3}$ |
| | | $10^{-2}$ | 9706 | (213) | 2604 | (67) | $5.78 \times 10^{-4}$ | 34232 | (318) | $1.83 \times 10^{-2}$ |
| | | $10^{-3}$ | 7999 | (3) | 2248 | (5) | $5.78 \times 10^{-4}$ | 31429 | (4) | $1.82 \times 10^{-3}$ |
| | | $10^{-4}$ | 7996 | (2) | 2205 | (0) | $5.78 \times 10^{-4}$ | 31429 | (5) | $1.78 \times 10^{-3}$ |
| | | $10^{-5}$ | 8014 | (3) | 2217 | (0) | $5.78 \times 10^{-4}$ | 31430 | (4) | $1.77 \times 10^{-3}$ |
| | | $10^{-6}$ | 8008 | (1) | 2259 | (0) | $5.78 \times 10^{-4}$ | 31450 | (4) | $1.77 \times 10^{-3}$ |
| | | $10^{-7}$ | 8020 | (2) | 2679 | (0) | $5.78 \times 10^{-4}$ | 31462 | (4) | $1.77 \times 10^{-3}$ |
| | | $10^{-8}$ | 8050 | (1) | 4149 | (0) | $5.78 \times 10^{-4}$ | 31468 | (3) | $1.77 \times 10^{-3}$ |

Table 3: Performance of general purpose schemes: Number of function evaluations (#FE), rejected steps (#R), and $L^2$ error of the density for the Taylor Green vortex (5.3), the isentropic vortex (5.4), and the flow with source term (5.5) using polynomials of degree $p = 3$.

| | | | TGV (5.3) | | Isent. vortex (5.4) | | | Source term (5.5) | | |
|---|---|---|---|---|---|---|---|---|---|---|
| Scheme | $\beta$ | `tol` | #FE | #R | #FE | #R | Error | #FE | #R | Error |
| BS3(2)3$_F$ | (0.60, −0.20, 0.00) | $10^{-1}$ | 12230 | (878) | 3073 | (304) | $2.31 \times 10^{-4}$ | 43178 | (2212) | $6.83 \times 10^{-2}$ |
| | | $10^{-2}$ | 10107 | (5) | 2952 | (174) | $1.53 \times 10^{-4}$ | 36733 | (6) | $8.48 \times 10^{-3}$ |
| | | $10^{-3}$ | 10144 | (5) | 2679 | (1) | $1.28 \times 10^{-4}$ | 36671 | (5) | $1.80 \times 10^{-4}$ |
| | | $10^{-4}$ | 10159 | (5) | 2679 | (0) | $1.26 \times 10^{-4}$ | 36708 | (4) | $2.84 \times 10^{-5}$ |
| | | $10^{-5}$ | 10162 | (4) | 2685 | (0) | $1.26 \times 10^{-4}$ | 36765 | (4) | $2.65 \times 10^{-5}$ |
| | | $10^{-6}$ | 10164 | (2) | 3069 | (0) | $1.25 \times 10^{-4}$ | 36792 | (4) | $2.65 \times 10^{-5}$ |
| | | $10^{-7}$ | 10164 | (1) | 6576 | (0) | $1.25 \times 10^{-4}$ | 36801 | (3) | $2.64 \times 10^{-5}$ |
| | | $10^{-8}$ | 10636 | (82) | 14142 | (0) | $1.24 \times 10^{-4}$ | 37656 | (1) | $2.64 \times 10^{-5}$ |
| BS5(4)7$_F$ | (0.28, −0.23, 0.00) | $10^{-1}$ | 16400 | (173) | 4378 | (50) | $1.26 \times 10^{-4}$ | 63970 | (553) | $1.92 \times 10^{-2}$ |
| | | $10^{-2}$ | 16440 | (150) | 4376 | (43) | $1.47 \times 10^{-4}$ | 66856 | (450) | $2.05 \times 10^{-2}$ |
| | | $10^{-3}$ | 16446 | (129) | 4321 | (34) | $1.27 \times 10^{-4}$ | 56749 | (65) | $1.28 \times 10^{-2}$ |
| | | $10^{-4}$ | 14932 | (2) | 4479 | (27) | $1.27 \times 10^{-4}$ | 53785 | (3) | $2.45 \times 10^{-3}$ |
| | | $10^{-5}$ | 14933 | (2) | 3951 | (0) | $1.25 \times 10^{-4}$ | 54091 | (5) | $2.02 \times 10^{-3}$ |
| | | $10^{-6}$ | 14940 | (2) | 3958 | (0) | $1.24 \times 10^{-4}$ | 54149 | (4) | $9.15 \times 10^{-4}$ |
| | | $10^{-7}$ | 14949 | (2) | 4000 | (0) | $1.24 \times 10^{-4}$ | 54090 | (4) | $2.64 \times 10^{-5}$ |
| | | $10^{-8}$ | 14948 | (1) | 4574 | (0) | $1.24 \times 10^{-4}$ | 54120 | (4) | $2.64 \times 10^{-5}$ |
| DP5(4)6$_F$ | (0.70, −0.40, 0.00) | $10^{-1}$ | 18694 | (601) | 4968 | (185) | $1.25 \times 10^{-4}$ | 67602 | (2011) | $7.54 \times 10^{-4}$ |
| | | $10^{-2}$ | 18946 | (471) | 4954 | (147) | $1.25 \times 10^{-4}$ | 66311 | (1151) | $2.76 \times 10^{-2}$ |
| | | $10^{-3}$ | 15448 | (3) | 4935 | (95) | $1.25 \times 10^{-4}$ | 55806 | (5) | $2.57 \times 10^{-4}$ |
| | | $10^{-4}$ | 15455 | (4) | 4083 | (1) | $1.24 \times 10^{-4}$ | 55860 | (4) | $2.65 \times 10^{-5}$ |
| | | $10^{-5}$ | 15467 | (4) | 4083 | (0) | $1.24 \times 10^{-4}$ | 55885 | (5) | $2.64 \times 10^{-5}$ |
| | | $10^{-6}$ | 15467 | (3) | 4089 | (0) | $1.24 \times 10^{-4}$ | 55911 | (4) | $2.64 \times 10^{-5}$ |
| | | $10^{-7}$ | 15473 | (3) | 4125 | (0) | $1.24 \times 10^{-4}$ | 55936 | (4) | $2.64 \times 10^{-5}$ |
| | | $10^{-8}$ | 15479 | (3) | 6093 | (0) | $1.24 \times 10^{-4}$ | 55960 | (4) | $2.64 \times 10^{-5}$ |

Table 4: Performance of general purpose schemes: Number of function evaluations (#FE), rejected steps (#R), and $L^2$ error of the density for the Taylor Green vortex (5.3), the isentropic vortex (5.4), and the flow with source term (5.5) using polynomials of degree $p = 4$.

| | | | TGV (5.3) | | Isent. vortex (5.4) | | | Source term (5.5) | | |
|---|---|---|---|---|---|---|---|---|---|---|
| Scheme | $\beta$ | `tol` | #FE | #R | #FE | #R | Error | #FE | #R | Error |
| $BS3(2)3_F$ | $(0.60, -0.20, 0.00)$ | $10^{-1}$ | 18398 | (1421) | 4858 | (486) | $2.13 \times 10^{-4}$ | 83227 | (4997) | $1.77 \times 10^{-1}$ |
| | | $10^{-2}$ | 16457 | (31) | 4550 | (283) | $1.34 \times 10^{-4}$ | 56214 | (8) | $7.32 \times 10^{-3}$ |
| | | $10^{-3}$ | 16555 | (6) | 4224 | (3) | $6.83 \times 10^{-5}$ | 56060 | (5) | $7.17 \times 10^{-5}$ |
| | | $10^{-4}$ | 16585 | (5) | 4221 | (1) | $1.20 \times 10^{-5}$ | 56151 | (5) | $1.07 \times 10^{-5}$ |
| | | $10^{-5}$ | 16603 | (5) | 4227 | (1) | $1.19 \times 10^{-5}$ | 56223 | (5) | $1.53 \times 10^{-6}$ |
| | | $10^{-6}$ | 16606 | (3) | 4230 | (0) | $1.19 \times 10^{-5}$ | 56271 | (5) | $9.36 \times 10^{-7}$ |
| | | $10^{-7}$ | 16614 | (3) | 6690 | (0) | $1.17 \times 10^{-5}$ | 56289 | (3) | $8.95 \times 10^{-7}$ |
| | | $10^{-8}$ | 18384 | (156) | 14385 | (0) | $1.16 \times 10^{-5}$ | 56601 | (2) | $6.57 \times 10^{-7}$ |
| $BS5(4)7_F$ | $(0.28, -0.23, 0.00)$ | $10^{-1}$ | 26740 | (293) | 6981 | (85) | $8.20 \times 10^{-5}$ | 96908 | (849) | $2.09 \times 10^{-2}$ |
| | | $10^{-2}$ | 26845 | (259) | 6957 | (71) | $1.49 \times 10^{-4}$ | 104630 | (691) | $2.74 \times 10^{-2}$ |
| | | $10^{-3}$ | 27120 | (227) | 6967 | (60) | $3.62 \times 10^{-5}$ | 86328 | (50) | $2.13 \times 10^{-2}$ |
| | | $10^{-4}$ | 24492 | (10) | 7045 | (47) | $7.00 \times 10^{-5}$ | 82497 | (3) | $1.22 \times 10^{-3}$ |
| | | $10^{-5}$ | 24438 | (5) | 6264 | (2) | $1.60 \times 10^{-4}$ | 82578 | (4) | $2.11 \times 10^{-5}$ |
| | | $10^{-6}$ | 24419 | (4) | 6212 | (0) | $1.16 \times 10^{-5}$ | 82632 | (2) | $1.05 \times 10^{-5}$ |
| | | $10^{-7}$ | 24433 | (4) | 6226 | (0) | $1.16 \times 10^{-5}$ | 82698 | (3) | $2.93 \times 10^{-6}$ |
| | | $10^{-8}$ | 24434 | (3) | 6268 | (0) | $1.16 \times 10^{-5}$ | 82741 | (3) | $5.18 \times 10^{-7}$ |
| $DP5(4)6_F$ | $(0.70, -0.40, 0.00)$ | $10^{-1}$ | 31777 | (1138) | 7829 | (291) | $8.51 \times 10^{-5}$ | 103055 | (3091) | $5.99 \times 10^{-4}$ |
| | | $10^{-2}$ | 30556 | (816) | 7621 | (232) | $4.90 \times 10^{-5}$ | 103442 | (2192) | $6.36 \times 10^{-3}$ |
| | | $10^{-3}$ | 30361 | (652) | 7675 | (165) | $9.57 \times 10^{-5}$ | 85268 | (6) | $1.55 \times 10^{-4}$ |
| | | $10^{-4}$ | 25245 | (5) | 6430 | (2) | $1.18 \times 10^{-5}$ | 85341 | (5) | $3.92 \times 10^{-6}$ |
| | | $10^{-5}$ | 25265 | (6) | 6430 | (1) | $1.16 \times 10^{-5}$ | 85402 | (4) | $9.56 \times 10^{-7}$ |
| | | $10^{-6}$ | 25271 | (5) | 6436 | (1) | $1.16 \times 10^{-5}$ | 85440 | (4) | $5.18 \times 10^{-7}$ |
| | | $10^{-7}$ | 25283 | (5) | 6442 | (1) | $1.16 \times 10^{-5}$ | 85495 | (3) | $5.18 \times 10^{-7}$ |
| | | $10^{-8}$ | 25283 | (3) | 6514 | (1) | $1.16 \times 10^{-5}$ | 85539 | (3) | $5.18 \times 10^{-7}$ |

Table 5: Performance of general purpose schemes: Number of function evaluations (#FE), rejected steps (#R), and $L^2$ error of the density for the Taylor Green vortex (5.3), the isentropic vortex (5.4), and the flow with source term (5.5) using polynomials of degree $p = 7$.

| | | | TGV (5.3) | | Isent. vortex (5.4) | | | Source term (5.5) | | |
|---|---|---|---|---|---|---|---|---|---|---|
| Scheme | $\beta$ | `tol` | #FE | #R | #FE | #R | Error | #FE | #R | Error |
| BS3(2)3$_F$ | $(0.60, -0.20, 0.00)$ | $10^{-1}$ | 56627 | (5180) | 10574 | (1300) | $1.81 \times 10^{-4}$ | 168548 | (10319) | $5.39 \times 10^{-2}$ |
| | | $10^{-2}$ | 50593 | (3015) | 13036 | (964) | $2.35 \times 10^{-4}$ | 132663 | (170) | $6.16 \times 10^{-3}$ |
| | | $10^{-3}$ | 45141 | (4) | 10826 | (4) | $2.78 \times 10^{-4}$ | 132408 | (7) | $7.81 \times 10^{-5}$ |
| | | $10^{-4}$ | 45288 | (7) | 10830 | (4) | $7.58 \times 10^{-6}$ | 132564 | (7) | $1.17 \times 10^{-6}$ |
| | | $10^{-5}$ | 45345 | (6) | 10833 | (3) | $1.41 \times 10^{-7}$ | 132642 | (6) | $1.32 \times 10^{-7}$ |
| | | $10^{-6}$ | 45390 | (6) | 10833 | (1) | $1.20 \times 10^{-7}$ | 132681 | (5) | $7.07 \times 10^{-8}$ |
| | | $10^{-7}$ | 45408 | (4) | 10833 | (0) | $1.14 \times 10^{-7}$ | 132714 | (4) | $5.76 \times 10^{-8}$ |
| | | $10^{-8}$ | 48834 | (115) | 14244 | (0) | $7.83 \times 10^{-8}$ | 132735 | (3) | $5.61 \times 10^{-8}$ |
| BS5(4)7$_F$ | $(0.28, -0.23, 0.00)$ | $10^{-1}$ | 73700 | (888) | 17693 | (224) | $9.43 \times 10^{-5}$ | 231596 | (2085) | $5.68 \times 10^{-3}$ |
| | | $10^{-2}$ | 73807 | (766) | 17738 | (193) | $4.50 \times 10^{-5}$ | 237762 | (1687) | $3.99 \times 10^{-3}$ |
| | | $10^{-3}$ | 74342 | (675) | 17831 | (165) | $1.06 \times 10^{-4}$ | 215488 | (590) | $3.60 \times 10^{-3}$ |
| | | $10^{-4}$ | 76509 | (559) | 17872 | (136) | $3.02 \times 10^{-5}$ | 194921 | (5) | $7.78 \times 10^{-4}$ |
| | | $10^{-5}$ | 66604 | (4) | 17259 | (77) | $2.33 \times 10^{-5}$ | 195023 | (6) | $9.92 \times 10^{-6}$ |
| | | $10^{-6}$ | 66693 | (4) | 15926 | (1) | $6.61 \times 10^{-6}$ | 195024 | (4) | $4.23 \times 10^{-6}$ |
| | | $10^{-7}$ | 66737 | (4) | 15935 | (1) | $3.03 \times 10^{-5}$ | 195090 | (4) | $4.08 \times 10^{-9}$ |
| | | $10^{-8}$ | 66775 | (4) | 15935 | (0) | $6.94 \times 10^{-8}$ | 195128 | (5) | $3.08 \times 10^{-9}$ |
| DP5(4)6$_F$ | $(0.70, -0.40, 0.00)$ | $10^{-1}$ | 92391 | (4202) | 21081 | (874) | $3.32 \times 10^{-5}$ | 249403 | (7646) | $1.10 \times 10^{-3}$ |
| | | $10^{-2}$ | 86089 | (2850) | 19826 | (620) | $1.15 \times 10^{-4}$ | 245052 | (5213) | $4.10 \times 10^{-3}$ |
| | | $10^{-3}$ | 82866 | (2146) | 19873 | (483) | $1.70 \times 10^{-5}$ | 202702 | (89) | $3.37 \times 10^{-4}$ |
| | | $10^{-4}$ | 69228 | (4) | 16467 | (3) | $2.51 \times 10^{-5}$ | 201634 | (6) | $4.37 \times 10^{-6}$ |
| | | $10^{-5}$ | 68932 | (4) | 16459 | (1) | $8.92 \times 10^{-7}$ | 201642 | (6) | $3.63 \times 10^{-8}$ |
| | | $10^{-6}$ | 69002 | (5) | 16479 | (2) | $6.81 \times 10^{-8}$ | 201674 | (5) | $2.80 \times 10^{-9}$ |
| | | $10^{-7}$ | 69028 | (4) | 16479 | (1) | $6.80 \times 10^{-8}$ | 201712 | (5) | $1.85 \times 10^{-9}$ |
| | | $10^{-8}$ | 69136 | (4) | 16485 | (1) | $6.80 \times 10^{-8}$ | 201718 | (4) | $1.31 \times 10^{-9}$ |

## 2.2 SSP methods

Table 6: Performance of SSP schemes: Number of function evaluations (#FE), rejected steps (#R), and $L^2$ error of the density for the inviscid Taylor Green vortex (5.3), the isentropic vortex (5.4), and the flow with source term (5.5) using polynomials of degree $p = 2$.

| | | | TGV (5.3) | | Isent. vortex (5.4) | | | Source term (5.5) | | |
|---|---|---|---|---|---|---|---|---|---|---|
| Scheme | $\beta$ | `tol` | #FE | #R | #FE | #R | Error | #FE | #R | Error |
| SSP3(2)3[3S*$_+$] | $(0.70, -0.37, 0.05)$ | $10^{-3}$ | 5243 | (2) | 1445 | (1) | $5.76 \times 10^{-4}$ | 20620 | (5) | $1.77 \times 10^{-3}$ |
| | | $10^{-4}$ | 5252 | (1) | 1451 | (0) | $5.77 \times 10^{-4}$ | 20660 | (4) | $1.77 \times 10^{-3}$ |
| | | $10^{-5}$ | 5261 | (3) | 1646 | (0) | $5.77 \times 10^{-4}$ | 20681 | (3) | $1.77 \times 10^{-3}$ |
| | | $10^{-6}$ | 5297 | (3) | 3488 | (0) | $5.78 \times 10^{-4}$ | 20711 | (2) | $1.77 \times 10^{-3}$ |
| | | $10^{-7}$ | 5387 | (2) | 7490 | (0) | $5.78 \times 10^{-4}$ | 21440 | (1) | $1.77 \times 10^{-3}$ |
| | | $10^{-8}$ | 6758 | (40) | 16109 | (0) | $5.78 \times 10^{-4}$ | 25310 | (1) | $1.77 \times 10^{-3}$ |
| SSP3(2)4[3S*$_+$] | $(0.55, -0.27, 0.05)$ | $10^{-3}$ | 3426 | (3) | 1250 | (1) | $5.74 \times 10^{-4}$ | 20614 | (5) | $1.78 \times 10^{-3}$ |
| | | $10^{-4}$ | 3426 | (4) | 1266 | (0) | $5.76 \times 10^{-4}$ | 20618 | (3) | $1.77 \times 10^{-3}$ |
| | | $10^{-5}$ | 3438 | (1) | 1902 | (0) | $5.78 \times 10^{-4}$ | 20638 | (3) | $1.77 \times 10^{-3}$ |
| | | $10^{-6}$ | 3490 | (2) | 4066 | (0) | $5.78 \times 10^{-4}$ | 20722 | (2) | $1.77 \times 10^{-3}$ |
| | | $10^{-7}$ | 3910 | (13) | 8730 | (0) | $5.78 \times 10^{-4}$ | 21726 | (2) | $1.77 \times 10^{-3}$ |
| | | $10^{-8}$ | 7406 | (32) | 18774 | (0) | $5.78 \times 10^{-4}$ | 27146 | (0) | $1.77 \times 10^{-3}$ |

Table 7: Performance of SSP schemes: Number of function evaluations (#FE), rejected steps (#R), and $L^2$ error of the density for the Taylor Green vortex (5.3), the isentropic vortex (5.4), and the flow with source term (5.5) using polynomials of degree $p = 3$.

| | | | TGV (5.3) | | Isent. vortex (5.4) | | | Source term (5.5) | | |
|---|---|---|---|---|---|---|---|---|---|---|
| Scheme | $\beta$ | `tol` | #FE | #R | #FE | #R | Error | #FE | #R | Error |
| SSP3(2)3[3S*$_+$] | $(0.70, -0.37, 0.05)$ | $10^{-3}$ | 10136 | (4) | 2678 | (1) | $1.26 \times 10^{-4}$ | 36637 | (5) | $4.04 \times 10^{-5}$ |
| | | $10^{-4}$ | 10154 | (4) | 2681 | (0) | $1.26 \times 10^{-4}$ | 36713 | (5) | $2.91 \times 10^{-5}$ |
| | | $10^{-5}$ | 10163 | (4) | 2687 | (0) | $1.26 \times 10^{-4}$ | 36767 | (4) | $2.65 \times 10^{-5}$ |
| | | $10^{-6}$ | 10169 | (3) | 4595 | (0) | $1.25 \times 10^{-4}$ | 36791 | (3) | $2.65 \times 10^{-5}$ |
| | | $10^{-7}$ | 10190 | (13) | 9890 | (0) | $1.24 \times 10^{-4}$ | 37010 | (4) | $2.64 \times 10^{-5}$ |
| | | $10^{-8}$ | 14162 | (76) | 21293 | (0) | $1.24 \times 10^{-4}$ | 38996 | (1) | $2.64 \times 10^{-5}$ |
| SSP3(2)4[3S*$_+$] | $(0.55, -0.27, 0.05)$ | $10^{-3}$ | 6610 | (5) | 2150 | (1) | $1.27 \times 10^{-4}$ | 35149 | (4) | $3.57 \times 10^{-5}$ |
| | | $10^{-4}$ | 6610 | (3) | 2154 | (0) | $1.27 \times 10^{-4}$ | 35153 | (3) | $2.71 \times 10^{-5}$ |
| | | $10^{-5}$ | 6614 | (2) | 2486 | (0) | $1.26 \times 10^{-4}$ | 35210 | (4) | $2.66 \times 10^{-5}$ |
| | | $10^{-6}$ | 6618 | (5) | 5358 | (0) | $1.25 \times 10^{-4}$ | 35226 | (2) | $2.65 \times 10^{-5}$ |
| | | $10^{-7}$ | 7486 | (19) | 11530 | (0) | $1.24 \times 10^{-4}$ | 35650 | (5) | $2.64 \times 10^{-5}$ |
| | | $10^{-8}$ | 16242 | (41) | 24814 | (0) | $1.24 \times 10^{-4}$ | 38530 | (1) | $2.64 \times 10^{-5}$ |

Table 8: Performance of SSP schemes: Number of function evaluations (#FE), rejected steps (#R), and $L^2$ error of the density for the Taylor Green vortex (5.3), the isentropic vortex (5.4), and the flow with source term (5.5) using polynomials of degree $p = 4$.

| | | | TGV (5.3) | | Isent. vortex (5.4) | | | Source term (5.5) | | |
|---|---|---|---|---|---|---|---|---|---|---|
| Scheme | $\beta$ | `tol` | #FE | #R | #FE | #R | Error | #FE | #R | Error |
| SSP3(2)3[3S*$_+$] | $(0.70, -0.37, 0.05)$ | $10^{-3}$ | 16544 | (7) | 4223 | (3) | $2.53 \times 10^{-5}$ | 55999 | (6) | $3.84 \times 10^{-5}$ |
| | | $10^{-4}$ | 16580 | (6) | 4223 | (1) | $1.19 \times 10^{-5}$ | 56129 | (5) | $7.74 \times 10^{-6}$ |
| | | $10^{-5}$ | 16604 | (6) | 4220 | (0) | $1.19 \times 10^{-5}$ | 56219 | (5) | $1.55 \times 10^{-6}$ |
| | | $10^{-6}$ | 16610 | (4) | 4703 | (0) | $1.18 \times 10^{-5}$ | 56261 | (4) | $9.25 \times 10^{-7}$ |
| | | $10^{-7}$ | 16658 | (12) | 10133 | (0) | $1.17 \times 10^{-5}$ | 56294 | (4) | $8.92 \times 10^{-7}$ |
| | | $10^{-8}$ | 23771 | (157) | 21821 | (0) | $1.16 \times 10^{-5}$ | 57407 | (3) | $5.57 \times 10^{-7}$ |
| SSP3(2)4[3S*$_+$] | $(0.55, -0.27, 0.05)$ | $10^{-3}$ | 10782 | (6) | 3254 | (2) | $9.35 \times 10^{-5}$ | 52765 | (8) | $2.14 \times 10^{-5}$ |
| | | $10^{-4}$ | 10798 | (5) | 3254 | (1) | $1.36 \times 10^{-5}$ | 52817 | (9) | $2.85 \times 10^{-6}$ |
| | | $10^{-5}$ | 10806 | (4) | 3254 | (0) | $1.27 \times 10^{-5}$ | 52866 | (9) | $1.41 \times 10^{-6}$ |
| | | $10^{-6}$ | 10806 | (5) | 5486 | (0) | $1.18 \times 10^{-5}$ | 52890 | (5) | $1.19 \times 10^{-6}$ |
| | | $10^{-7}$ | 12538 | (34) | 11810 | (0) | $1.16 \times 10^{-5}$ | 52978 | (4) | $9.62 \times 10^{-7}$ |
| | | $10^{-8}$ | 26098 | (72) | 25430 | (0) | $1.16 \times 10^{-5}$ | 54750 | (3) | $5.54 \times 10^{-7}$ |

Table 9: Performance of SSP schemes: Number of function evaluations (#FE), rejected steps (#R), and $L^2$ error of the density for the Taylor Green vortex (5.3), the isentropic vortex (5.4), and the flow with source term (5.5) using polynomials of degree $p = 7$.

| | | | TGV (5.3) | | Isent. vortex (5.4) | | | Source term (5.5) | | |
|---|---|---|---|---|---|---|---|---|---|---|
| Scheme | $\beta$ | `tol` | #FE | #R | #FE | #R | Error | #FE | #R | Error |
| SSP3(2)3[3S*$_+$] | $(0.70, -0.37, 0.05)$ | $10^{-3}$ | 45173 | (9) | 10823 | (4) | $1.44 \times 10^{-4}$ | 132328 | (6) | $2.18 \times 10^{-5}$ |
| | | $10^{-4}$ | 45281 | (7) | 10823 | (3) | $2.71 \times 10^{-6}$ | 132497 | (6) | $8.71 \times 10^{-7}$ |
| | | $10^{-5}$ | 45350 | (7) | 10829 | (2) | $1.40 \times 10^{-7}$ | 132578 | (5) | $2.21 \times 10^{-7}$ |
| | | $10^{-6}$ | 45389 | (6) | 10835 | (1) | $1.17 \times 10^{-7}$ | 132647 | (4) | $9.11 \times 10^{-8}$ |
| | | $10^{-7}$ | 45611 | (15) | 10841 | (0) | $1.13 \times 10^{-7}$ | 132707 | (4) | $5.84 \times 10^{-8}$ |
| | | $10^{-8}$ | 58640 | (148) | 21656 | (0) | $6.87 \times 10^{-8}$ | 132740 | (4) | $5.60 \times 10^{-8}$ |
| SSP3(2)4[3S*$_+$] | $(0.55, -0.27, 0.05)$ | $10^{-3}$ | 29421 | (6) | 7678 | (3) | $2.02 \times 10^{-4}$ | 120594 | (6) | $4.30 \times 10^{-5}$ |
| | | $10^{-4}$ | 29490 | (6) | 7666 | (1) | $8.33 \times 10^{-6}$ | 120718 | (5) | $1.10 \times 10^{-6}$ |
| | | $10^{-5}$ | 29534 | (6) | 7674 | (1) | $3.36 \times 10^{-7}$ | 120786 | (5) | $1.56 \times 10^{-7}$ |
| | | $10^{-6}$ | 29542 | (6) | 7682 | (1) | $3.10 \times 10^{-7}$ | 120826 | (5) | $9.28 \times 10^{-8}$ |
| | | $10^{-7}$ | 33514 | (18) | 11722 | (0) | $1.08 \times 10^{-7}$ | 120838 | (3) | $8.78 \times 10^{-8}$ |
| | | $10^{-8}$ | 58982 | (64) | 25238 | (0) | $6.84 \times 10^{-8}$ | 120994 | (4) | $7.28 \times 10^{-8}$ |

## 2.3 Low-storage methods

Table 10: Performance of low-storage schemes: Number of function evaluations (#FE), rejected steps (#R), and $L^2$ error of the density for the inviscid Taylor Green vortex (5.3), the isentropic vortex (5.4), and the flow with source term (5.5) using polynomials of degree $p = 2$.

| | | | TGV (5.3) | | Isent. vortex (5.4) | | | Source term (5.5) | | |
|---|---|---|---|---|---|---|---|---|---|---|
| Scheme | $\beta$ | `tol` | #FE | #R | #FE | #R | Error | #FE | #R | Error |
| KCL3(2)4[2R$_+$]C | $(0.50, -0.35, 0.10)$ | $10^{-1}$ | 7609 | (331) | 2149 | (113) | $5.79 \times 10^{-4}$ | 30576 | (939) | $2.05 \times 10^{-2}$ |
| | | $10^{-2}$ | 6305 | (2) | 2057 | (73) | $5.79 \times 10^{-4}$ | 24812 | (4) | $2.02 \times 10^{-3}$ |
| | | $10^{-3}$ | 6309 | (1) | 1738 | (0) | $5.78 \times 10^{-4}$ | 24849 | (5) | $1.78 \times 10^{-3}$ |
| | | $10^{-4}$ | 6322 | (1) | 1750 | (0) | $5.78 \times 10^{-4}$ | 24857 | (3) | $1.77 \times 10^{-3}$ |
| | | $10^{-5}$ | 6326 | (1) | 1874 | (0) | $5.78 \times 10^{-4}$ | 24886 | (3) | $1.77 \times 10^{-3}$ |
| | | $10^{-6}$ | 6370 | (2) | 3714 | (0) | $5.78 \times 10^{-4}$ | 24906 | (4) | $1.77 \times 10^{-3}$ |
| | | $10^{-7}$ | 6458 | (1) | 7954 | (0) | $5.78 \times 10^{-4}$ | 25582 | (1) | $1.77 \times 10^{-3}$ |
| | | $10^{-8}$ | 7578 | (28) | 17094 | (0) | $5.78 \times 10^{-4}$ | 29270 | (0) | $1.77 \times 10^{-3}$ |
| KCL4(3)5[2R$_+$]C | $(0.29, -0.24, 0.02)$ | $10^{-1}$ | 5269 | (80) | 1690 | (22) | $5.79 \times 10^{-4}$ | 28561 | (289) | $4.62 \times 10^{-2}$ |
| | | $10^{-2}$ | 5319 | (65) | 1734 | (15) | $5.81 \times 10^{-4}$ | 24033 | (16) | $6.29 \times 10^{-3}$ |
| | | $10^{-3}$ | 5345 | (53) | 1412 | (0) | $5.79 \times 10^{-4}$ | 23835 | (2) | $1.76 \times 10^{-3}$ |
| | | $10^{-4}$ | 4572 | (3) | 1437 | (0) | $5.79 \times 10^{-4}$ | 23877 | (3) | $2.18 \times 10^{-3}$ |
| | | $10^{-5}$ | 4897 | (65) | 1522 | (0) | $5.79 \times 10^{-4}$ | 23902 | (5) | $1.77 \times 10^{-3}$ |
| | | $10^{-6}$ | 4582 | (0) | 2112 | (0) | $5.78 \times 10^{-4}$ | 23907 | (3) | $1.77 \times 10^{-3}$ |
| | | $10^{-7}$ | 4652 | (0) | 3647 | (0) | $5.78 \times 10^{-4}$ | 23922 | (3) | $1.77 \times 10^{-3}$ |
| | | $10^{-8}$ | 5047 | (4) | 6387 | (0) | $5.78 \times 10^{-4}$ | 24032 | (1) | $1.77 \times 10^{-3}$ |
| KCL4(3)5[3R$_+$]C | $(0.41, -0.28, 0.08)$ | $10^{-1}$ | 5471 | (164) | 1798 | (53) | $5.79 \times 10^{-4}$ | 27665 | (563) | $1.02 \times 10^{-1}$ |
| | | $10^{-2}$ | 5500 | (131) | 1768 | (33) | $5.77 \times 10^{-4}$ | 23640 | (3) | $3.99 \times 10^{-3}$ |
| | | $10^{-3}$ | 4676 | (10) | 1402 | (0) | $5.79 \times 10^{-4}$ | 23755 | (2) | $1.77 \times 10^{-3}$ |
| | | $10^{-4}$ | 4652 | (9) | 1417 | (0) | $5.79 \times 10^{-4}$ | 23792 | (2) | $1.78 \times 10^{-3}$ |
| | | $10^{-5}$ | 4587 | (42) | 1472 | (0) | $5.79 \times 10^{-4}$ | 23817 | (4) | $1.77 \times 10^{-3}$ |
| | | $10^{-6}$ | 4592 | (20) | 2057 | (0) | $5.78 \times 10^{-4}$ | 23827 | (4) | $1.77 \times 10^{-3}$ |
| | | $10^{-7}$ | 4802 | (1) | 3602 | (0) | $5.78 \times 10^{-4}$ | 23837 | (3) | $1.77 \times 10^{-3}$ |
| | | $10^{-8}$ | 5032 | (2) | 6362 | (0) | $5.78 \times 10^{-4}$ | 23937 | (1) | $1.77 \times 10^{-3}$ |
| KCL5(4)9[2R$_+$]S | $(0.49, -0.34, 0.10)$ | $10^{-1}$ | 8883 | (164) | 2552 | (52) | $5.81 \times 10^{-4}$ | 38417 | (510) | $5.89 \times 10^{-2}$ |
| | | $10^{-2}$ | 6907 | (36) | 2431 | (36) | $5.76 \times 10^{-4}$ | 30329 | (3) | $9.55 \times 10^{-3}$ |
| | | $10^{-3}$ | 6310 | (3) | 2045 | (0) | $5.78 \times 10^{-4}$ | 30371 | (3) | $1.77 \times 10^{-3}$ |
| | | $10^{-4}$ | 6302 | (2) | 2063 | (0) | $5.78 \times 10^{-4}$ | 30385 | (3) | $1.77 \times 10^{-3}$ |
| | | $10^{-5}$ | 6320 | (3) | 2108 | (0) | $5.78 \times 10^{-4}$ | 30374 | (3) | $1.77 \times 10^{-3}$ |
| | | $10^{-6}$ | 6329 | (3) | 2432 | (0) | $5.78 \times 10^{-4}$ | 30386 | (3) | $1.77 \times 10^{-3}$ |
| | | $10^{-7}$ | 6365 | (3) | 3719 | (0) | $5.78 \times 10^{-4}$ | 30395 | (3) | $1.77 \times 10^{-3}$ |
| | | $10^{-8}$ | 6716 | (11) | 5798 | (0) | $5.78 \times 10^{-4}$ | 30413 | (2) | $1.77 \times 10^{-3}$ |

Table 11: Performance of low-storage schemes: Number of function evaluations (#FE), rejected steps (#R), and $L^2$ error of the density for the Taylor Green vortex (5.3), the isentropic vortex (5.4), and the flow with source term (5.5) using polynomials of degree $p = 3$.

| | | | TGV (5.3) | | Isent. vortex (5.4) | | | Source term (5.5) | | |
|---|---|---|---|---|---|---|---|---|---|---|
| Scheme | $\beta$ | `tol` | #FE | #R | #FE | #R | Error | #FE | #R | Error |
| KCL3(2)4[2R+]C | $(0.50, -0.35, 0.10)$ | $10^{-1}$ | 14771 | (644) | 4002 | (211) | $1.26 \times 10^{-4}$ | 52906 | (2028) | $7.36 \times 10^{-5}$ |
| | | $10^{-2}$ | 14659 | (378) | 3836 | (142) | $1.25 \times 10^{-4}$ | 54020 | (1235) | $1.33 \times 10^{-3}$ |
| | | $10^{-3}$ | 12193 | (3) | 3222 | (1) | $1.25 \times 10^{-4}$ | 44172 | (4) | $2.88 \times 10^{-5}$ |
| | | $10^{-4}$ | 12210 | (3) | 3230 | (1) | $1.25 \times 10^{-4}$ | 44176 | (3) | $2.65 \times 10^{-5}$ |
| | | $10^{-5}$ | 12226 | (3) | 3238 | (0) | $1.25 \times 10^{-4}$ | 44250 | (5) | $2.64 \times 10^{-5}$ |
| | | $10^{-6}$ | 12230 | (2) | 4790 | (0) | $1.24 \times 10^{-4}$ | 44274 | (4) | $2.64 \times 10^{-5}$ |
| | | $10^{-7}$ | 12254 | (5) | 10286 | (0) | $1.24 \times 10^{-4}$ | 44434 | (3) | $2.64 \times 10^{-5}$ |
| | | $10^{-8}$ | 15054 | (62) | 22122 | (0) | $1.24 \times 10^{-4}$ | 46314 | (1) | $2.64 \times 10^{-5}$ |
| KCL4(3)5[2R+]C | $(0.29, -0.24, 0.02)$ | $10^{-1}$ | 10241 | (164) | 2878 | (41) | $1.31 \times 10^{-4}$ | 47198 | (516) | $3.46 \times 10^{-2}$ |
| | | $10^{-2}$ | 10285 | (134) | 2869 | (29) | $1.26 \times 10^{-4}$ | 39357 | (3) | $2.31 \times 10^{-3}$ |
| | | $10^{-3}$ | 10408 | (114) | 2397 | (0) | $1.26 \times 10^{-4}$ | 39440 | (3) | $4.35 \times 10^{-5}$ |
| | | $10^{-4}$ | 11231 | (109) | 2397 | (0) | $1.25 \times 10^{-4}$ | 39507 | (4) | $2.65 \times 10^{-5}$ |
| | | $10^{-5}$ | 9270 | (69) | 2417 | (0) | $1.25 \times 10^{-4}$ | 39542 | (4) | $2.64 \times 10^{-5}$ |
| | | $10^{-6}$ | 8922 | (15) | 2832 | (0) | $1.25 \times 10^{-4}$ | 39547 | (2) | $2.64 \times 10^{-5}$ |
| | | $10^{-7}$ | 8847 | (2) | 4942 | (0) | $1.24 \times 10^{-4}$ | 39577 | (3) | $2.64 \times 10^{-5}$ |
| | | $10^{-8}$ | 9487 | (7) | 8707 | (0) | $1.24 \times 10^{-4}$ | 39597 | (3) | $2.64 \times 10^{-5}$ |
| KCL4(3)5[3R+]C | $(0.41, -0.28, 0.08)$ | $10^{-1}$ | 10625 | (325) | 3015 | (93) | $1.26 \times 10^{-4}$ | 49004 | (1078) | $1.47 \times 10^{-1}$ |
| | | $10^{-2}$ | 10636 | (249) | 3014 | (66) | $1.24 \times 10^{-4}$ | 40218 | (78) | $5.91 \times 10^{-3}$ |
| | | $10^{-3}$ | 9096 | (9) | 2427 | (1) | $1.25 \times 10^{-4}$ | 39284 | (3) | $9.36 \times 10^{-5}$ |
| | | $10^{-4}$ | 8782 | (64) | 2417 | (0) | $1.25 \times 10^{-4}$ | 39345 | (4) | $2.91 \times 10^{-5}$ |
| | | $10^{-5}$ | 9037 | (27) | 2427 | (0) | $1.25 \times 10^{-4}$ | 39386 | (5) | $2.64 \times 10^{-5}$ |
| | | $10^{-6}$ | 8937 | (29) | 2807 | (0) | $1.25 \times 10^{-4}$ | 39412 | (5) | $2.64 \times 10^{-5}$ |
| | | $10^{-7}$ | 9152 | (4) | 4942 | (0) | $1.24 \times 10^{-4}$ | 39427 | (4) | $2.64 \times 10^{-5}$ |
| | | $10^{-8}$ | 9537 | (9) | 8742 | (0) | $1.24 \times 10^{-4}$ | 39437 | (3) | $2.64 \times 10^{-5}$ |
| KCL5(4)9[2R+]S | $(0.49, -0.34, 0.10)$ | $10^{-1}$ | 17116 | (320) | 5086 | (115) | $1.31 \times 10^{-4}$ | 66213 | (952) | $2.03 \times 10^{-2}$ |
| | | $10^{-2}$ | 17483 | (288) | 4653 | (82) | $1.31 \times 10^{-4}$ | 52730 | (3) | $3.61 \times 10^{-3}$ |
| | | $10^{-3}$ | 12177 | (5) | 3719 | (1) | $1.29 \times 10^{-4}$ | 52772 | (4) | $2.83 \times 10^{-5}$ |
| | | $10^{-4}$ | 12169 | (3) | 3710 | (0) | $1.24 \times 10^{-4}$ | 52793 | (4) | $2.64 \times 10^{-5}$ |
| | | $10^{-5}$ | 12179 | (5) | 3719 | (0) | $1.24 \times 10^{-4}$ | 52765 | (4) | $2.64 \times 10^{-5}$ |
| | | $10^{-6}$ | 12179 | (4) | 3755 | (0) | $1.24 \times 10^{-4}$ | 52775 | (3) | $2.64 \times 10^{-5}$ |
| | | $10^{-7}$ | 12179 | (4) | 5366 | (0) | $1.24 \times 10^{-4}$ | 52766 | (2) | $2.64 \times 10^{-5}$ |
| | | $10^{-8}$ | 13142 | (16) | 8327 | (0) | $1.24 \times 10^{-4}$ | 52796 | (2) | $2.64 \times 10^{-5}$ |

Table 12: Performance of low-storage schemes: Number of function evaluations (#FE), rejected steps (#R), and $L^2$ error of the density for the Taylor Green vortex (5.3), the isentropic vortex (5.4), and the flow with source term (5.5) using polynomials of degree $p = 4$.

| | | | TGV (5.3) | | Isent. vortex (5.4) | | | Source term (5.5) | | |
|---|---|---|---|---|---|---|---|---|---|---|
| Scheme | $\beta$ | `tol` | #FE | #R | #FE | #R | Error | #FE | #R | Error |
| KCL3(2)4[2R$_+$]C | $(0.50, -0.35, 0.10)$ | $10^{-1}$ | 24169 | (1070) | 6316 | (333) | $1.41 \times 10^{-5}$ | 81066 | (3097) | $7.92 \times 10^{-5}$ |
| | | $10^{-2}$ | 23795 | (654) | 6059 | (227) | $1.31 \times 10^{-5}$ | 67454 | (5) | $3.04 \times 10^{-4}$ |
| | | $10^{-3}$ | 19905 | (5) | 5069 | (1) | $1.57 \times 10^{-5}$ | 67536 | (4) | $2.11 \times 10^{-5}$ |
| | | $10^{-4}$ | 19950 | (5) | 5078 | (1) | $1.16 \times 10^{-5}$ | 67601 | (5) | $2.41 \times 10^{-6}$ |
| | | $10^{-5}$ | 19966 | (3) | 5082 | (1) | $1.16 \times 10^{-5}$ | 67645 | (4) | $8.64 \times 10^{-7}$ |
| | | $10^{-6}$ | 19986 | (4) | 5102 | (0) | $1.16 \times 10^{-5}$ | 67710 | (5) | $5.19 \times 10^{-7}$ |
| | | $10^{-7}$ | 19990 | (2) | 10462 | (0) | $1.16 \times 10^{-5}$ | 67726 | (3) | $5.18 \times 10^{-7}$ |
| | | $10^{-8}$ | 25698 | (178) | 22514 | (0) | $1.16 \times 10^{-5}$ | 68694 | (2) | $5.18 \times 10^{-7}$ |
| KCL4(3)5[2R$_+$]C | $(0.29, -0.24, 0.02)$ | $10^{-1}$ | 17133 | (298) | 4296 | (65) | $4.51 \times 10^{-5}$ | 69437 | (795) | $3.20 \times 10^{-2}$ |
| | | $10^{-2}$ | 16969 | (245) | 4381 | (54) | $8.91 \times 10^{-5}$ | 58014 | (5) | $2.06 \times 10^{-3}$ |
| | | $10^{-3}$ | 17080 | (205) | 4578 | (48) | $1.31 \times 10^{-4}$ | 58120 | (4) | $2.16 \times 10^{-5}$ |
| | | $10^{-4}$ | 18297 | (164) | 3672 | (0) | $1.21 \times 10^{-5}$ | 58226 | (6) | $1.00 \times 10^{-5}$ |
| | | $10^{-5}$ | 14981 | (100) | 3677 | (0) | $1.16 \times 10^{-5}$ | 58282 | (5) | $1.11 \times 10^{-6}$ |
| | | $10^{-6}$ | 14581 | (26) | 3702 | (0) | $1.16 \times 10^{-5}$ | 58322 | (5) | $5.19 \times 10^{-7}$ |
| | | $10^{-7}$ | 14462 | (12) | 4962 | (0) | $1.16 \times 10^{-5}$ | 58337 | (4) | $5.18 \times 10^{-7}$ |
| | | $10^{-8}$ | 18427 | (9) | 8762 | (0) | $1.16 \times 10^{-5}$ | 58357 | (4) | $5.18 \times 10^{-7}$ |
| KCL4(3)5[3R$_+$]C | $(0.41, -0.28, 0.08)$ | $10^{-1}$ | 17836 | (606) | 4612 | (160) | $1.52 \times 10^{-4}$ | 69224 | (1635) | $7.14 \times 10^{-2}$ |
| | | $10^{-2}$ | 17392 | (425) | 4457 | (104) | $2.00 \times 10^{-4}$ | 60464 | (217) | $1.20 \times 10^{-2}$ |
| | | $10^{-3}$ | 16237 | (223) | 4503 | (64) | $1.03 \times 10^{-4}$ | 57818 | (4) | $5.22 \times 10^{-5}$ |
| | | $10^{-4}$ | 14542 | (41) | 3797 | (0) | $1.16 \times 10^{-5}$ | 57910 | (4) | $2.44 \times 10^{-6}$ |
| | | $10^{-5}$ | 14352 | (96) | 3797 | (0) | $1.16 \times 10^{-5}$ | 57972 | (4) | $5.67 \times 10^{-7}$ |
| | | $10^{-6}$ | 14742 | (40) | 3817 | (0) | $1.16 \times 10^{-5}$ | 58022 | (6) | $5.16 \times 10^{-7}$ |
| | | $10^{-7}$ | 14832 | (22) | 4977 | (0) | $1.16 \times 10^{-5}$ | 58047 | (6) | $5.18 \times 10^{-7}$ |
| | | $10^{-8}$ | 16767 | (9) | 8817 | (0) | $1.16 \times 10^{-5}$ | 58047 | (4) | $5.18 \times 10^{-7}$ |
| KCL5(4)9[2R$_+$]S | $(0.49, -0.34, 0.10)$ | $10^{-1}$ | 29611 | (611) | 7925 | (186) | $1.20 \times 10^{-5}$ | 102210 | (1486) | $5.41 \times 10^{-2}$ |
| | | $10^{-2}$ | 30647 | (527) | 7342 | (131) | $2.96 \times 10^{-5}$ | 81668 | (52) | $3.21 \times 10^{-3}$ |
| | | $10^{-3}$ | 19842 | (4) | 7432 | (114) | $1.85 \times 10^{-4}$ | 80812 | (4) | $2.28 \times 10^{-5}$ |
| | | $10^{-4}$ | 19854 | (3) | 5753 | (1) | $1.29 \times 10^{-5}$ | 80862 | (4) | $5.74 \times 10^{-7}$ |
| | | $10^{-5}$ | 19874 | (5) | 5744 | (0) | $1.16 \times 10^{-5}$ | 80815 | (3) | $5.18 \times 10^{-7}$ |
| | | $10^{-6}$ | 19865 | (4) | 5753 | (0) | $1.16 \times 10^{-5}$ | 80854 | (4) | $5.18 \times 10^{-7}$ |
| | | $10^{-7}$ | 19874 | (5) | 5789 | (0) | $1.16 \times 10^{-5}$ | 80874 | (3) | $5.18 \times 10^{-7}$ |
| | | $10^{-8}$ | 23933 | (14) | 8750 | (0) | $1.16 \times 10^{-5}$ | 80903 | (4) | $5.18 \times 10^{-7}$ |

Table 13: Performance of low-storage schemes: Number of function evaluations (#FE), rejected steps (#R), and $L^2$ error of the density for the Taylor Green vortex (5.3), the isentropic vortex (5.4), and the flow with source term (5.5) using polynomials of degree $p = 7$.

| | | | TGV (5.3) | | Isent. vortex (5.4) | | | Source term (5.5) | | |
|---|---|---|---|---|---|---|---|---|---|---|
| Scheme | $\beta$ | `tol` | #FE | #R | #FE | #R | Error | #FE | #R | Error |
| KCL3(2)4[2R$_+$]C | $(0.50, -0.35, 0.10)$ | $10^{-1}$ | 67242 | (3557) | 16558 | (975) | $3.01 \times 10^{-5}$ | 190669 | (7073) | $2.47 \times 10^{-3}$ |
| | | $10^{-2}$ | 64798 | (2358) | 15752 | (687) | $1.78 \times 10^{-5}$ | 158370 | (4) | $2.87 \times 10^{-4}$ |
| | | $10^{-3}$ | 54501 | (23) | 15605 | (430) | $1.69 \times 10^{-5}$ | 159245 | (5) | $4.91 \times 10^{-6}$ |
| | | $10^{-4}$ | 54505 | (5) | 13021 | (2) | $1.80 \times 10^{-6}$ | 159482 | (5) | $2.04 \times 10^{-6}$ |
| | | $10^{-5}$ | 54578 | (6) | 13030 | (2) | $7.08 \times 10^{-8}$ | 159590 | (6) | $4.03 \times 10^{-8}$ |
| | | $10^{-6}$ | 54610 | (5) | 13034 | (1) | $6.81 \times 10^{-8}$ | 159634 | (5) | $9.08 \times 10^{-9}$ |
| | | $10^{-7}$ | 54706 | (11) | 13042 | (0) | $6.80 \times 10^{-8}$ | 159658 | (4) | $1.29 \times 10^{-9}$ |
| | | $10^{-8}$ | 67318 | (210) | 22286 | (0) | $6.80 \times 10^{-8}$ | 159678 | (3) | $1.20 \times 10^{-9}$ |
| KCL4(3)5[2R$_+$]C | $(0.29, -0.24, 0.02)$ | $10^{-1}$ | 45711 | (874) | 11485 | (245) | $1.59 \times 10^{-4}$ | 155453 | (1959) | $1.60 \times 10^{-2}$ |
| | | $10^{-2}$ | 46082 | (739) | 11314 | (197) | $7.43 \times 10^{-5}$ | 137839 | (311) | $4.57 \times 10^{-3}$ |
| | | $10^{-3}$ | 47228 | (647) | 11374 | (157) | $6.52 \times 10^{-5}$ | 131586 | (5) | $2.14 \times 10^{-5}$ |
| | | $10^{-4}$ | 49952 | (514) | 11444 | (116) | $1.04 \times 10^{-4}$ | 131798 | (3) | $4.03 \times 10^{-7}$ |
| | | $10^{-5}$ | 40336 | (41) | 9835 | (16) | $6.97 \times 10^{-5}$ | 131940 | (4) | $6.25 \times 10^{-7}$ |
| | | $10^{-6}$ | 39600 | (31) | 9417 | (0) | $6.82 \times 10^{-8}$ | 132031 | (4) | $9.70 \times 10^{-10}$ |
| | | $10^{-7}$ | 39471 | (5) | 9422 | (0) | $6.84 \times 10^{-8}$ | 132087 | (4) | $8.88 \times 10^{-10}$ |
| | | $10^{-8}$ | 49182 | (35) | 9452 | (0) | $6.79 \times 10^{-8}$ | 132122 | (4) | $1.05 \times 10^{-9}$ |
| KCL4(3)5[3R$_+$]C | $(0.41, -0.28, 0.08)$ | $10^{-1}$ | 50833 | (2054) | 11980 | (500) | $3.27 \times 10^{-5}$ | 157577 | (3902) | $1.91 \times 10^{-2}$ |
| | | $10^{-2}$ | 47985 | (1353) | 11451 | (395) | $4.00 \times 10^{-5}$ | 149988 | (1608) | $1.66 \times 10^{-2}$ |
| | | $10^{-3}$ | 48955 | (1227) | 11454 | (273) | $8.63 \times 10^{-5}$ | 131125 | (5) | $4.97 \times 10^{-5}$ |
| | | $10^{-4}$ | 40074 | (96) | 9736 | (4) | $5.30 \times 10^{-5}$ | 131348 | (5) | $7.44 \times 10^{-7}$ |
| | | $10^{-5}$ | 39770 | (165) | 9737 | (3) | $1.03 \times 10^{-6}$ | 131484 | (5) | $2.65 \times 10^{-7}$ |
| | | $10^{-6}$ | 40292 | (87) | 9732 | (1) | $6.81 \times 10^{-8}$ | 131576 | (5) | $1.10 \times 10^{-9}$ |
| | | $10^{-7}$ | 40442 | (82) | 9737 | (1) | $6.79 \times 10^{-8}$ | 131632 | (5) | $8.91 \times 10^{-10}$ |
| | | $10^{-8}$ | 44802 | (69) | 9762 | (0) | $6.79 \times 10^{-8}$ | 131662 | (4) | $1.06 \times 10^{-9}$ |
| KCL5(4)9[2R$_+$]S | $(0.49, -0.34, 0.10)$ | $10^{-1}$ | 88831 | (1990) | 20329 | (474) | $6.03 \times 10^{-5}$ | 238316 | (3797) | $2.12 \times 10^{-2}$ |
| | | $10^{-2}$ | 89287 | (2431) | 19044 | (386) | $2.12 \times 10^{-4}$ | 194685 | (187) | $1.45 \times 10^{-3}$ |
| | | $10^{-3}$ | 55976 | (107) | 19358 | (341) | $1.67 \times 10^{-4}$ | 191686 | (4) | $5.57 \times 10^{-5}$ |
| | | $10^{-4}$ | 54200 | (3) | 15361 | (129) | $7.97 \times 10^{-5}$ | 191628 | (4) | $3.51 \times 10^{-7}$ |
| | | $10^{-5}$ | 54241 | (3) | 15806 | (175) | $2.42 \times 10^{-6}$ | 191670 | (4) | $3.46 \times 10^{-8}$ |
| | | $10^{-6}$ | 54250 | (5) | 16247 | (223) | $6.85 \times 10^{-8}$ | 191699 | (4) | $1.69 \times 10^{-9}$ |
| | | $10^{-7}$ | 54350 | (5) | 16463 | (239) | $6.80 \times 10^{-8}$ | 191718 | (4) | $1.31 \times 10^{-9}$ |
| | | $10^{-8}$ | 62776 | (11) | 15365 | (122) | $6.80 \times 10^{-8}$ | 191720 | (3) | $1.32 \times 10^{-9}$ |

Table 14: Performance of optimized low-storage schemes: Number of function evaluations (#FE), rejected steps (#R), and $L^2$ error of the density for the inviscid Taylor Green vortex (5.3), the isentropic vortex (5.4), and the flow with source term (5.5) using polynomials of degree $p = 2$.

| | | | TGV (5.3) | | Isent. vortex (5.4) | | | Source term (5.5) | | |
|---|---|---|---|---|---|---|---|---|---|---|
| Scheme | $\beta$ | `tol` | #FE | #R | #FE | #R | Error | #FE | #R | Error |
| RK3(2)5[3S*$_+$] | $(0.64, -0.31, 0.04)$ | $10^{-1}$ | 4821 | (306) | 1640 | (103) | $5.69 \times 10^{-4}$ | 26195 | (1309) | $6.07 \times 10^{-2}$ |
| | | $10^{-2}$ | 6463 | (435) | 1621 | (84) | $8.03 \times 10^{-4}$ | 20833 | (327) | $7.94 \times 10^{-2}$ |
| | | $10^{-3}$ | 4450 | (3) | 1399 | (33) | $5.70 \times 10^{-4}$ | 19640 | (2) | $2.50 \times 10^{-3}$ |
| | | $10^{-4}$ | 4467 | (2) | 1237 | (1) | $5.75 \times 10^{-4}$ | 19670 | (3) | $1.78 \times 10^{-3}$ |
| | | $10^{-5}$ | 4467 | (2) | 1262 | (0) | $5.77 \times 10^{-4}$ | 19692 | (3) | $1.77 \times 10^{-3}$ |
| | | $10^{-6}$ | 4487 | (2) | 2042 | (0) | $5.78 \times 10^{-4}$ | 19702 | (2) | $1.77 \times 10^{-3}$ |
| | | $10^{-7}$ | 4532 | (1) | 4367 | (0) | $5.78 \times 10^{-4}$ | 19842 | (4) | $1.77 \times 10^{-3}$ |
| | | $10^{-8}$ | 4782 | (0) | 9367 | (0) | $5.78 \times 10^{-4}$ | 21132 | (2) | $1.77 \times 10^{-3}$ |
| RK3(2)5$_\mathrm{F}$[3S*$_+$] | $(0.70, -0.23, 0.00)$ | $10^{-1}$ | 5197 | (282) | 1583 | (87) | $5.79 \times 10^{-4}$ | 23091 | (735) | $1.48 \times 10^{-1}$ |
| | | $10^{-2}$ | 4454 | (3) | 1437 | (39) | $5.69 \times 10^{-4}$ | 19667 | (13) | $3.22 \times 10^{-3}$ |
| | | $10^{-3}$ | 4465 | (2) | 1234 | (1) | $5.75 \times 10^{-4}$ | 19687 | (5) | $1.79 \times 10^{-3}$ |
| | | $10^{-4}$ | 4464 | (1) | 1238 | (0) | $5.76 \times 10^{-4}$ | 19696 | (3) | $1.77 \times 10^{-3}$ |
| | | $10^{-5}$ | 4469 | (1) | 1308 | (0) | $5.77 \times 10^{-4}$ | 19690 | (2) | $1.77 \times 10^{-3}$ |
| | | $10^{-6}$ | 4494 | (1) | 2258 | (0) | $5.78 \times 10^{-4}$ | 19711 | (3) | $1.77 \times 10^{-3}$ |
| | | $10^{-7}$ | 4543 | (0) | 4648 | (0) | $5.78 \times 10^{-4}$ | 19843 | (5) | $1.77 \times 10^{-3}$ |
| | | $10^{-8}$ | 5255 | (32) | 9863 | (0) | $5.78 \times 10^{-4}$ | 21051 | (3) | $1.77 \times 10^{-3}$ |
| RK4(3)9[3S*$_+$] | $(0.25, -0.12, 0.00)$ | $10^{-1}$ | 5501 | (110) | 1610 | (28) | $5.80 \times 10^{-4}$ | 25152 | (366) | $5.73 \times 10^{-3}$ |
| | | $10^{-2}$ | 5202 | (90) | 1591 | (20) | $5.80 \times 10^{-4}$ | 25605 | (300) | $5.05 \times 10^{-3}$ |
| | | $10^{-3}$ | 5488 | (94) | 1582 | (13) | $5.80 \times 10^{-4}$ | 25465 | (210) | $1.35 \times 10^{-2}$ |
| | | $10^{-4}$ | 5557 | (75) | 1316 | (0) | $5.80 \times 10^{-4}$ | 19323 | (11) | $1.78 \times 10^{-3}$ |
| | | $10^{-5}$ | 4205 | (1) | 1478 | (0) | $5.79 \times 10^{-4}$ | 18992 | (1) | $1.78 \times 10^{-3}$ |
| | | $10^{-6}$ | 4241 | (0) | 2414 | (0) | $5.78 \times 10^{-4}$ | 19019 | (2) | $1.77 \times 10^{-3}$ |
| | | $10^{-7}$ | 4358 | (0) | 4178 | (0) | $5.78 \times 10^{-4}$ | 19046 | (1) | $1.77 \times 10^{-3}$ |
| | | $10^{-8}$ | 5276 | (0) | 7328 | (0) | $5.78 \times 10^{-4}$ | 19397 | (0) | $1.77 \times 10^{-3}$ |
| RK4(3)9$_\mathrm{F}$[3S*$_+$] | $(0.38, -0.18, 0.01)$ | $10^{-1}$ | 5519 | (139) | 1660 | (41) | $5.80 \times 10^{-4}$ | 25698 | (500) | $9.60 \times 10^{-3}$ |
| | | $10^{-2}$ | 5664 | (133) | 1594 | (27) | $5.80 \times 10^{-4}$ | 25907 | (405) | $8.04 \times 10^{-3}$ |
| | | $10^{-3}$ | 5699 | (107) | 1592 | (18) | $5.81 \times 10^{-4}$ | 19771 | (40) | $2.70 \times 10^{-3}$ |
| | | $10^{-4}$ | 4198 | (1) | 1290 | (0) | $5.80 \times 10^{-4}$ | 18990 | (2) | $1.78 \times 10^{-3}$ |
| | | $10^{-5}$ | 4207 | (1) | 1371 | (0) | $5.80 \times 10^{-4}$ | 18984 | (1) | $1.77 \times 10^{-3}$ |
| | | $10^{-6}$ | 4234 | (1) | 1947 | (0) | $5.78 \times 10^{-4}$ | 19004 | (2) | $1.77 \times 10^{-3}$ |
| | | $10^{-7}$ | 4309 | (4) | 3297 | (0) | $5.78 \times 10^{-4}$ | 19013 | (2) | $1.77 \times 10^{-3}$ |
| | | $10^{-8}$ | 5091 | (12) | 5736 | (0) | $5.78 \times 10^{-4}$ | 19155 | (0) | $1.77 \times 10^{-3}$ |
| RK5(4)10[3S*$_+$] | $(0.47, -0.20, 0.06)$ | $10^{-1}$ | 6665 | (185) | 2060 | (54) | $5.84 \times 10^{-4}$ | 32633 | (733) | $9.20 \times 10^{-3}$ |
| | | $10^{-2}$ | 7167 | (183) | 1867 | (33) | $5.78 \times 10^{-4}$ | 32119 | (525) | $4.67 \times 10^{-2}$ |
| | | $10^{-3}$ | 5347 | (2) | 1837 | (20) | $5.78 \times 10^{-4}$ | 24077 | (4) | $3.74 \times 10^{-3}$ |
| | | $10^{-4}$ | 5362 | (2) | 1492 | (0) | $5.78 \times 10^{-4}$ | 24132 | (3) | $1.78 \times 10^{-3}$ |
| | | $10^{-5}$ | 5372 | (2) | 1512 | (0) | $5.78 \times 10^{-4}$ | 24107 | (3) | $1.78 \times 10^{-3}$ |
| | | $10^{-6}$ | 5362 | (1) | 1592 | (0) | $5.78 \times 10^{-4}$ | 24098 | (1) | $1.77 \times 10^{-3}$ |
| | | $10^{-7}$ | 5382 | (1) | 2132 | (0) | $5.78 \times 10^{-4}$ | 24112 | (1) | $1.77 \times 10^{-3}$ |
| | | $10^{-8}$ | 5412 | (0) | 3162 | (0) | $5.78 \times 10^{-4}$ | 24132 | (2) | $1.77 \times 10^{-3}$ |
| RK5(4)10$_\mathrm{F}$[3S*$_+$] | $(0.45, -0.13, 0.00)$ | $10^{-1}$ | 6986 | (184) | 2054 | (47) | $5.76 \times 10^{-4}$ | 32710 | (609) | $5.73 \times 10^{-2}$ |
| | | $10^{-2}$ | 5369 | (5) | 1911 | (29) | $5.84 \times 10^{-4}$ | 24379 | (27) | $5.09 \times 10^{-3}$ |
| | | $10^{-3}$ | 5370 | (3) | 1483 | (0) | $5.78 \times 10^{-4}$ | 24119 | (3) | $1.80 \times 10^{-3}$ |
| | | $10^{-4}$ | 5375 | (2) | 1503 | (0) | $5.78 \times 10^{-4}$ | 24134 | (3) | $1.78 \times 10^{-3}$ |
| | | $10^{-5}$ | 5364 | (1) | 1533 | (0) | $5.78 \times 10^{-4}$ | 24112 | (2) | $1.77 \times 10^{-3}$ |
| | | $10^{-6}$ | 5374 | (1) | 1683 | (0) | $5.78 \times 10^{-4}$ | 24136 | (3) | $1.77 \times 10^{-3}$ |
| | | $10^{-7}$ | 5383 | (0) | 2403 | (0) | $5.78 \times 10^{-4}$ | 24114 | (1) | $1.77 \times 10^{-3}$ |
| | | $10^{-8}$ | 5521 | (8) | 3693 | (0) | $5.78 \times 10^{-4}$ | 24135 | (2) | $1.77 \times 10^{-3}$ |

Table 15: Performance of optimized low-storage schemes: Number of function evaluations (#FE), rejected steps (#R), and $L^2$ error of the density for the Taylor Green vortex (5.3), the isentropic vortex (5.4), and the flow with source term (5.5) using polynomials of degree $p = 3$.

| | | | TGV (5.3) | | Isent. vortex (5.4) | | | Source term (5.5) | | |
|---|---|---|---|---|---|---|---|---|---|---|
| Scheme | $\beta$ | `tol` | #FE | #R | #FE | #R | Error | #FE | #R | Error |
| RK3(2)5[3S*$_+$] | $(0.64, -0.31, 0.04)$ | $10^{-1}$ | 11683 | (831) | 2783 | (188) | $1.43 \times 10^{-4}$ | 44093 | (2380) | $5.97 \times 10^{-2}$ |
| | | $10^{-2}$ | 9716 | (530) | 2644 | (144) | $1.31 \times 10^{-4}$ | 40615 | (1357) | $5.93 \times 10^{-2}$ |
| | | $10^{-3}$ | 8668 | (17) | 3200 | (190) | $1.30 \times 10^{-4}$ | 31963 | (5) | $1.60 \times 10^{-3}$ |
| | | $10^{-4}$ | 8627 | (3) | 2277 | (1) | $1.30 \times 10^{-4}$ | 31960 | (3) | $3.41 \times 10^{-5}$ |
| | | $10^{-5}$ | 8622 | (1) | 2287 | (1) | $1.27 \times 10^{-4}$ | 31961 | (2) | $2.75 \times 10^{-5}$ |
| | | $10^{-6}$ | 8632 | (1) | 2617 | (0) | $1.26 \times 10^{-4}$ | 32002 | (4) | $2.66 \times 10^{-5}$ |
| | | $10^{-7}$ | 8647 | (2) | 5647 | (0) | $1.25 \times 10^{-4}$ | 32007 | (2) | $2.66 \times 10^{-5}$ |
| | | $10^{-8}$ | 8777 | (14) | 12142 | (0) | $1.24 \times 10^{-4}$ | 32657 | (1) | $2.64 \times 10^{-5}$ |
| RK3(2)5$_F$[3S*$_+$] | $(0.70, -0.23, 0.00)$ | $10^{-1}$ | 10614 | (568) | 2766 | (163) | $1.31 \times 10^{-4}$ | 41871 | (1630) | $3.95 \times 10^{-2}$ |
| | | $10^{-2}$ | 8613 | (4) | 2797 | (134) | $1.30 \times 10^{-4}$ | 31949 | (10) | $1.97 \times 10^{-3}$ |
| | | $10^{-3}$ | 8637 | (4) | 2279 | (1) | $1.29 \times 10^{-4}$ | 31976 | (5) | $3.82 \times 10^{-5}$ |
| | | $10^{-4}$ | 8630 | (2) | 2284 | (1) | $1.27 \times 10^{-4}$ | 31997 | (4) | $2.66 \times 10^{-5}$ |
| | | $10^{-5}$ | 8635 | (2) | 2288 | (0) | $1.27 \times 10^{-4}$ | 32029 | (6) | $2.66 \times 10^{-5}$ |
| | | $10^{-6}$ | 8634 | (1) | 3078 | (0) | $1.25 \times 10^{-4}$ | 32016 | (3) | $2.66 \times 10^{-5}$ |
| | | $10^{-7}$ | 8685 | (7) | 6378 | (0) | $1.25 \times 10^{-4}$ | 32026 | (3) | $2.66 \times 10^{-5}$ |
| | | $10^{-8}$ | 10511 | (78) | 13573 | (0) | $1.24 \times 10^{-4}$ | 32635 | (2) | $2.64 \times 10^{-5}$ |
| RK4(3)9[3S*$_+$] | $(0.25, -0.12, 0.00)$ | $10^{-1}$ | 10297 | (216) | 2738 | (48) | $1.26 \times 10^{-4}$ | 44589 | (624) | $3.23 \times 10^{-3}$ |
| | | $10^{-2}$ | 11298 | (206) | 2740 | (39) | $1.25 \times 10^{-4}$ | 44112 | (460) | $1.42 \times 10^{-3}$ |
| | | $10^{-3}$ | 10335 | (170) | 2716 | (26) | $1.26 \times 10^{-4}$ | 44506 | (366) | $1.84 \times 10^{-3}$ |
| | | $10^{-4}$ | 10749 | (143) | 2747 | (17) | $1.25 \times 10^{-4}$ | 33222 | (17) | $7.11 \times 10^{-5}$ |
| | | $10^{-5}$ | 8163 | (4) | 2225 | (0) | $1.25 \times 10^{-4}$ | 32721 | (2) | $2.68 \times 10^{-5}$ |
| | | $10^{-6}$ | 8102 | (1) | 3161 | (0) | $1.25 \times 10^{-4}$ | 32753 | (3) | $2.64 \times 10^{-5}$ |
| | | $10^{-7}$ | 8102 | (0) | 5555 | (0) | $1.24 \times 10^{-4}$ | 32753 | (2) | $2.64 \times 10^{-5}$ |
| | | $10^{-8}$ | 10424 | (0) | 9821 | (0) | $1.24 \times 10^{-4}$ | 32798 | (1) | $2.64 \times 10^{-5}$ |
| RK4(3)9$_F$[3S*$_+$] | $(0.38, -0.18, 0.01)$ | $10^{-1}$ | 10388 | (270) | 2788 | (70) | $1.26 \times 10^{-4}$ | 44894 | (874) | $7.56 \times 10^{-3}$ |
| | | $10^{-2}$ | 11977 | (336) | 2755 | (53) | $1.26 \times 10^{-4}$ | 43633 | (645) | $1.90 \times 10^{-3}$ |
| | | $10^{-3}$ | 11072 | (296) | 2706 | (34) | $1.26 \times 10^{-4}$ | 37789 | (246) | $8.29 \times 10^{-4}$ |
| | | $10^{-4}$ | 8110 | (2) | 2421 | (10) | $1.25 \times 10^{-4}$ | 32725 | (4) | $2.87 \times 10^{-5}$ |
| | | $10^{-5}$ | 8105 | (2) | 2190 | (0) | $1.25 \times 10^{-4}$ | 32716 | (2) | $2.64 \times 10^{-5}$ |
| | | $10^{-6}$ | 8115 | (3) | 2658 | (0) | $1.25 \times 10^{-4}$ | 32748 | (3) | $2.64 \times 10^{-5}$ |
| | | $10^{-7}$ | 8105 | (2) | 4476 | (0) | $1.25 \times 10^{-4}$ | 32747 | (2) | $2.64 \times 10^{-5}$ |
| | | $10^{-8}$ | 10939 | (28) | 7797 | (0) | $1.24 \times 10^{-4}$ | 32737 | (1) | $2.64 \times 10^{-5}$ |
| RK5(4)10[3S*$_+$] | $(0.47, -0.20, 0.06)$ | $10^{-1}$ | 12520 | (358) | 3448 | (95) | $1.26 \times 10^{-4}$ | 53323 | (1144) | $3.20 \times 10^{-2}$ |
| | | $10^{-2}$ | 13928 | (360) | 3203 | (60) | $1.28 \times 10^{-4}$ | 51553 | (731) | $3.45 \times 10^{-2}$ |
| | | $10^{-3}$ | 10712 | (34) | 3235 | (43) | $1.26 \times 10^{-4}$ | 39530 | (24) | $8.26 \times 10^{-4}$ |
| | | $10^{-4}$ | 10348 | (3) | 2742 | (1) | $1.42 \times 10^{-4}$ | 39179 | (4) | $3.06 \times 10^{-5}$ |
| | | $10^{-5}$ | 10361 | (3) | 2742 | (0) | $1.24 \times 10^{-4}$ | 39146 | (3) | $2.64 \times 10^{-5}$ |
| | | $10^{-6}$ | 10362 | (2) | 2762 | (0) | $1.24 \times 10^{-4}$ | 39157 | (3) | $2.64 \times 10^{-5}$ |
| | | $10^{-7}$ | 10352 | (1) | 3232 | (0) | $1.24 \times 10^{-4}$ | 39159 | (2) | $2.64 \times 10^{-5}$ |
| | | $10^{-8}$ | 10992 | (40) | 4782 | (0) | $1.24 \times 10^{-4}$ | 39162 | (1) | $2.64 \times 10^{-5}$ |
| RK5(4)10$_F$[3S*$_+$] | $(0.45, -0.13, 0.00)$ | $10^{-1}$ | 13523 | (357) | 3422 | (77) | $1.25 \times 10^{-4}$ | 53751 | (934) | $4.64 \times 10^{-2}$ |
| | | $10^{-2}$ | 13347 | (276) | 3383 | (57) | $1.26 \times 10^{-4}$ | 40441 | (72) | $6.16 \times 10^{-3}$ |
| | | $10^{-3}$ | 10383 | (5) | 2744 | (1) | $1.54 \times 10^{-4}$ | 39159 | (4) | $8.54 \times 10^{-5}$ |
| | | $10^{-4}$ | 10374 | (4) | 2743 | (0) | $1.24 \times 10^{-4}$ | 39171 | (3) | $2.64 \times 10^{-5}$ |
| | | $10^{-5}$ | 10366 | (3) | 2764 | (1) | $1.24 \times 10^{-4}$ | 39161 | (3) | $2.64 \times 10^{-5}$ |
| | | $10^{-6}$ | 10365 | (2) | 2773 | (0) | $1.24 \times 10^{-4}$ | 39172 | (2) | $2.64 \times 10^{-5}$ |
| | | $10^{-7}$ | 10375 | (2) | 3613 | (0) | $1.24 \times 10^{-4}$ | 39186 | (3) | $2.64 \times 10^{-5}$ |
| | | $10^{-8}$ | 11039 | (26) | 5513 | (0) | $1.24 \times 10^{-4}$ | 39174 | (1) | $2.64 \times 10^{-5}$ |

Table 16: Performance of optimized low-storage schemes: Number of function evaluations (#FE), rejected steps (#R), and $L^2$ error of the density for the Taylor Green vortex (5.3), the isentropic vortex (5.4), and the flow with source term (5.5) using polynomials of degree $p = 4$.

| | | | TGV (5.3) | | Isent. vortex (5.4) | | | Source term (5.5) | | |
|---|---|---|---|---|---|---|---|---|---|---|
| Scheme | $\beta$ | `tol` | #FE | #R | #FE | #R | Error | #FE | #R | Error |
| RK3(2)5[3S*$_+$] | $(0.64, -0.31, 0.04)$ | $10^{-1}$ | 19308 | (1380) | 4554 | (349) | $1.36 \times 10^{-4}$ | 63446 | (3490) | $7.24 \times 10^{-3}$ |
| | | $10^{-2}$ | 15570 | (869) | 4262 | (266) | $2.83 \times 10^{-5}$ | 60398 | (2194) | $5.59 \times 10^{-2}$ |
| | | $10^{-3}$ | 14618 | (131) | 5372 | (369) | $3.19 \times 10^{-5}$ | 47959 | (5) | $3.87 \times 10^{-3}$ |
| | | $10^{-4}$ | 14097 | (5) | 3587 | (2) | $3.76 \times 10^{-5}$ | 47816 | (4) | $4.40 \times 10^{-5}$ |
| | | $10^{-5}$ | 14107 | (4) | 3592 | (2) | $1.23 \times 10^{-5}$ | 47826 | (3) | $1.63 \times 10^{-6}$ |
| | | $10^{-6}$ | 14102 | (2) | 3597 | (0) | $1.23 \times 10^{-5}$ | 47837 | (2) | $1.43 \times 10^{-6}$ |
| | | $10^{-7}$ | 14112 | (1) | 5747 | (0) | $1.17 \times 10^{-5}$ | 47867 | (3) | $1.40 \times 10^{-6}$ |
| | | $10^{-8}$ | 14392 | (15) | 12367 | (0) | $1.16 \times 10^{-5}$ | 48122 | (3) | $8.91 \times 10^{-7}$ |
| RK3(2)5$_F$[3S*$_+$] | $(0.70, -0.23, 0.00)$ | $10^{-1}$ | 16598 | (926) | 4213 | (275) | $1.19 \times 10^{-4}$ | 65141 | (2951) | $1.79 \times 10^{-2}$ |
| | | $10^{-2}$ | 15591 | (355) | 4414 | (232) | $5.13 \times 10^{-5}$ | 47881 | (5) | $3.58 \times 10^{-3}$ |
| | | $10^{-3}$ | 14098 | (5) | 3589 | (2) | $2.37 \times 10^{-5}$ | 47786 | (5) | $4.63 \times 10^{-5}$ |
| | | $10^{-4}$ | 14107 | (4) | 3595 | (2) | $1.23 \times 10^{-5}$ | 47832 | (4) | $1.54 \times 10^{-6}$ |
| | | $10^{-5}$ | 14122 | (4) | 3594 | (1) | $1.23 \times 10^{-5}$ | 47846 | (3) | $1.43 \times 10^{-6}$ |
| | | $10^{-6}$ | 14115 | (2) | 3603 | (0) | $1.23 \times 10^{-5}$ | 47866 | (3) | $1.40 \times 10^{-6}$ |
| | | $10^{-7}$ | 14183 | (10) | 6578 | (0) | $1.17 \times 10^{-5}$ | 47865 | (2) | $1.40 \times 10^{-6}$ |
| | | $10^{-8}$ | 19774 | (146) | 14033 | (0) | $1.16 \times 10^{-5}$ | 48095 | (2) | $9.19 \times 10^{-7}$ |
| RK4(3)9[3S*$_+$] | $(0.25, -0.12, 0.00)$ | $10^{-1}$ | 16814 | (353) | 4210 | (80) | $1.87 \times 10^{-5}$ | 65943 | (979) | $8.99 \times 10^{-4}$ |
| | | $10^{-2}$ | 18372 | (350) | 4207 | (65) | $2.65 \times 10^{-5}$ | 66053 | (720) | $8.68 \times 10^{-4}$ |
| | | $10^{-3}$ | 17488 | (304) | 4177 | (48) | $1.45 \times 10^{-5}$ | 67855 | (590) | $1.04 \times 10^{-3}$ |
| | | $10^{-4}$ | 17580 | (244) | 4259 | (38) | $1.16 \times 10^{-5}$ | 50138 | (23) | $5.73 \times 10^{-5}$ |
| | | $10^{-5}$ | 13223 | (2) | 4122 | (26) | $1.17 \times 10^{-5}$ | 49586 | (2) | $1.56 \times 10^{-6}$ |
| | | $10^{-6}$ | 13220 | (1) | 3440 | (0) | $1.15 \times 10^{-5}$ | 49625 | (2) | $5.18 \times 10^{-7}$ |
| | | $10^{-7}$ | 13313 | (1) | 5555 | (0) | $1.16 \times 10^{-5}$ | 49646 | (2) | $5.18 \times 10^{-7}$ |
| | | $10^{-8}$ | 19433 | (0) | 9821 | (0) | $1.16 \times 10^{-5}$ | 49655 | (2) | $5.18 \times 10^{-7}$ |
| RK4(3)9$_F$[3S*$_+$] | $(0.38, -0.18, 0.01)$ | $10^{-1}$ | 17245 | (451) | 4351 | (117) | $5.87 \times 10^{-5}$ | 65797 | (1360) | $2.80 \times 10^{-4}$ |
| | | $10^{-2}$ | 21432 | (700) | 4117 | (85) | $1.18 \times 10^{-5}$ | 67044 | (1083) | $1.09 \times 10^{-3}$ |
| | | $10^{-3}$ | 19167 | (440) | 4341 | (81) | $1.60 \times 10^{-5}$ | 60016 | (514) | $1.39 \times 10^{-3}$ |
| | | $10^{-4}$ | 18110 | (350) | 4431 | (71) | $4.21 \times 10^{-5}$ | 49578 | (3) | $7.49 \times 10^{-6}$ |
| | | $10^{-5}$ | 13226 | (2) | 3387 | (0) | $1.15 \times 10^{-5}$ | 49580 | (2) | $6.26 \times 10^{-7}$ |
| | | $10^{-6}$ | 13245 | (3) | 3414 | (0) | $1.15 \times 10^{-5}$ | 49609 | (2) | $5.27 \times 10^{-7}$ |
| | | $10^{-7}$ | 13488 | (3) | 4584 | (0) | $1.16 \times 10^{-5}$ | 49631 | (2) | $5.18 \times 10^{-7}$ |
| | | $10^{-8}$ | 22636 | (25) | 7932 | (0) | $1.16 \times 10^{-5}$ | 49640 | (2) | $5.18 \times 10^{-7}$ |
| RK5(4)10[3S*$_+$] | $(0.47, -0.20, 0.06)$ | $10^{-1}$ | 20586 | (591) | 5138 | (150) | $8.71 \times 10^{-5}$ | 77624 | (1707) | $6.57 \times 10^{-3}$ |
| | | $10^{-2}$ | 22228 | (586) | 5506 | (149) | $1.48 \times 10^{-5}$ | 80960 | (1274) | $2.74 \times 10^{-2}$ |
| | | $10^{-3}$ | 17309 | (44) | 5248 | (112) | $3.30 \times 10^{-5}$ | 59314 | (111) | $8.04 \times 10^{-4}$ |
| | | $10^{-4}$ | 16927 | (4) | 4322 | (2) | $3.54 \times 10^{-5}$ | 57286 | (4) | $9.69 \times 10^{-6}$ |
| | | $10^{-5}$ | 16910 | (3) | 4312 | (1) | $1.17 \times 10^{-5}$ | 57263 | (4) | $5.31 \times 10^{-7}$ |
| | | $10^{-6}$ | 16922 | (3) | 4312 | (0) | $1.16 \times 10^{-5}$ | 57276 | (3) | $5.19 \times 10^{-7}$ |
| | | $10^{-7}$ | 16932 | (3) | 4332 | (0) | $1.16 \times 10^{-5}$ | 57298 | (3) | $5.18 \times 10^{-7}$ |
| | | $10^{-8}$ | 20532 | (41) | 5202 | (0) | $1.16 \times 10^{-5}$ | 57289 | (2) | $5.18 \times 10^{-7}$ |
| RK5(4)10$_F$[3S*$_+$] | $(0.45, -0.13, 0.00)$ | $10^{-1}$ | 21679 | (582) | 5396 | (149) | $1.90 \times 10^{-5}$ | 80389 | (1438) | $2.35 \times 10^{-2}$ |
| | | $10^{-2}$ | 21421 | (450) | 5803 | (148) | $1.17 \times 10^{-5}$ | 62966 | (282) | $2.86 \times 10^{-3}$ |
| | | $10^{-3}$ | 16919 | (4) | 4354 | (4) | $1.30 \times 10^{-4}$ | 57264 | (4) | $3.06 \times 10^{-5}$ |
| | | $10^{-4}$ | 16943 | (5) | 4325 | (2) | $1.17 \times 10^{-5}$ | 57322 | (6) | $8.20 \times 10^{-7}$ |
| | | $10^{-5}$ | 16925 | (3) | 4314 | (1) | $1.16 \times 10^{-5}$ | 57324 | (6) | $5.19 \times 10^{-7}$ |
| | | $10^{-6}$ | 16936 | (3) | 4313 | (0) | $1.16 \times 10^{-5}$ | 57314 | (5) | $5.18 \times 10^{-7}$ |
| | | $10^{-7}$ | 16947 | (4) | 4343 | (0) | $1.16 \times 10^{-5}$ | 57325 | (4) | $5.18 \times 10^{-7}$ |
| | | $10^{-8}$ | 20632 | (29) | 5843 | (0) | $1.16 \times 10^{-5}$ | 57359 | (6) | $5.18 \times 10^{-7}$ |

Table 17: Performance of optimized low-storage schemes: Number of function evaluations (#FE), rejected steps (#R), and $L^2$ error of the density for the Taylor Green vortex (5.3), the isentropic vortex (5.4), and the flow with source term (5.5) using polynomials of degree $p = 7$.

| | | | TGV (5.3) | | Isent. vortex (5.4) | | | Source term (5.5) | | |
|---|---|---|---|---|---|---|---|---|---|---|
| Scheme | $\beta$ | `tol` | #FE | #R | #FE | #R | Error | #FE | #R | Error |
| RK3(2)5[3S*$_+$] | $(0.64, -0.31, 0.04)$ | $10^{-1}$ | 51793 | (3731) | 11725 | (901) | $7.70 \times 10^{-5}$ | 139807 | (7933) | $8.40 \times 10^{-3}$ |
| | | $10^{-2}$ | 41977 | (2476) | 10375 | (655) | $8.15 \times 10^{-5}$ | 137082 | (5365) | $1.40 \times 10^{-2}$ |
| | | $10^{-3}$ | 49184 | (2482) | 9869 | (547) | $1.94 \times 10^{-5}$ | 114077 | (246) | $4.30 \times 10^{-3}$ |
| | | $10^{-4}$ | 38499 | (4) | 9206 | (3) | $1.92 \times 10^{-4}$ | 112705 | (4) | $3.58 \times 10^{-5}$ |
| | | $10^{-5}$ | 38555 | (4) | 9202 | (2) | $4.98 \times 10^{-6}$ | 112762 | (3) | $4.56 \times 10^{-6}$ |
| | | $10^{-6}$ | 38571 | (3) | 9207 | (2) | $1.94 \times 10^{-7}$ | 112802 | (3) | $1.04 \times 10^{-7}$ |
| | | $10^{-7}$ | 38592 | (3) | 9212 | (1) | $1.77 \times 10^{-7}$ | 112817 | (3) | $1.00 \times 10^{-7}$ |
| | | $10^{-8}$ | 39417 | (11) | 12247 | (0) | $9.64 \times 10^{-8}$ | 112817 | (2) | $1.00 \times 10^{-7}$ |
| RK3(2)5$_F$[3S*$_+$] | $(0.70, -0.23, 0.00)$ | $10^{-1}$ | 51969 | (3714) | 12442 | (894) | $1.80 \times 10^{-5}$ | 145309 | (6960) | $1.23 \times 10^{-2}$ |
| | | $10^{-2}$ | 49505 | (2529) | 11223 | (604) | $7.90 \times 10^{-5}$ | 113995 | (264) | $4.56 \times 10^{-3}$ |
| | | $10^{-3}$ | 38430 | (4) | 9216 | (4) | $1.87 \times 10^{-4}$ | 112591 | (4) | $3.25 \times 10^{-5}$ |
| | | $10^{-4}$ | 38528 | (4) | 9205 | (2) | $4.34 \times 10^{-6}$ | 112713 | (4) | $3.71 \times 10^{-7}$ |
| | | $10^{-5}$ | 38577 | (4) | 9210 | (2) | $2.01 \times 10^{-7}$ | 112781 | (4) | $1.17 \times 10^{-7}$ |
| | | $10^{-6}$ | 38596 | (3) | 9215 | (2) | $1.85 \times 10^{-7}$ | 112811 | (3) | $1.02 \times 10^{-7}$ |
| | | $10^{-7}$ | 38716 | (8) | 9219 | (1) | $1.76 \times 10^{-7}$ | 112831 | (3) | $1.00 \times 10^{-7}$ |
| | | $10^{-8}$ | 48922 | (119) | 13968 | (0) | $8.19 \times 10^{-8}$ | 112835 | (2) | $1.00 \times 10^{-7}$ |
| RK4(3)9[3S*$_+$] | $(0.25, -0.12, 0.00)$ | $10^{-1}$ | 46684 | (1045) | 10856 | (273) | $2.40 \times 10^{-6}$ | 148198 | (2617) | $4.41 \times 10^{-4}$ |
| | | $10^{-2}$ | 48002 | (957) | 11247 | (237) | $2.13 \times 10^{-5}$ | 146372 | (2176) | $4.49 \times 10^{-4}$ |
| | | $10^{-3}$ | 48660 | (847) | 11809 | (214) | $6.66 \times 10^{-6}$ | 151502 | (2107) | $1.56 \times 10^{-4}$ |
| | | $10^{-4}$ | 48310 | (759) | 11323 | (192) | $8.30 \times 10^{-6}$ | 141040 | (1266) | $2.61 \times 10^{-4}$ |
| | | $10^{-5}$ | 49168 | (574) | 11539 | (149) | $9.41 \times 10^{-6}$ | 110412 | (67) | $5.50 \times 10^{-6}$ |
| | | $10^{-6}$ | 36149 | (3) | 8648 | (2) | $6.99 \times 10^{-8}$ | 108770 | (3) | $1.29 \times 10^{-8}$ |
| | | $10^{-7}$ | 36683 | (2) | 8651 | (1) | $6.78 \times 10^{-8}$ | 108780 | (3) | $4.77 \times 10^{-9}$ |
| | | $10^{-8}$ | 50285 | (2) | 8804 | (0) | $6.78 \times 10^{-8}$ | 108793 | (2) | $5.86 \times 10^{-10}$ |
| RK4(3)9$_F$[3S*$_+$] | $(0.38, -0.18, 0.01)$ | $10^{-1}$ | 54111 | (1565) | 11570 | (374) | $1.43 \times 10^{-7}$ | 149530 | (3590) | $3.13 \times 10^{-4}$ |
| | | $10^{-2}$ | 54435 | (1751) | 11129 | (289) | $8.42 \times 10^{-5}$ | 154405 | (3507) | $1.39 \times 10^{-4}$ |
| | | $10^{-3}$ | 51699 | (1158) | 12808 | (367) | $1.22 \times 10^{-6}$ | 146873 | (2226) | $2.41 \times 10^{-4}$ |
| | | $10^{-4}$ | 51550 | (1174) | 12583 | (296) | $1.62 \times 10^{-5}$ | 117523 | (502) | $2.37 \times 10^{-5}$ |
| | | $10^{-5}$ | 36728 | (30) | 9858 | (73) | $3.28 \times 10^{-5}$ | 108904 | (7) | $1.89 \times 10^{-7}$ |
| | | $10^{-6}$ | 36172 | (5) | 8645 | (2) | $6.87 \times 10^{-8}$ | 108855 | (3) | $8.45 \times 10^{-10}$ |
| | | $10^{-7}$ | 37246 | (5) | 8653 | (1) | $6.82 \times 10^{-8}$ | 108859 | (2) | $7.17 \times 10^{-10}$ |
| | | $10^{-8}$ | 57840 | (12) | 8661 | (0) | $6.79 \times 10^{-8}$ | 108879 | (3) | $5.96 \times 10^{-10}$ |
| RK5(4)10[3S*$_+$] | $(0.47, -0.20, 0.06)$ | $10^{-3}$ | 61458 | (1520) | 14705 | (380) | $8.35 \times 10^{-6}$ | 191136 | (3073) | $8.25 \times 10^{-3}$ |
| | | $10^{-4}$ | 46309 | (13) | 11494 | (44) | $3.36 \times 10^{-5}$ | 135466 | (27) | $2.91 \times 10^{-5}$ |
| | | $10^{-5}$ | 46237 | (4) | 11052 | (3) | $3.11 \times 10^{-6}$ | 135072 | (5) | $7.28 \times 10^{-8}$ |
| | | $10^{-6}$ | 46203 | (4) | 11042 | (2) | $6.87 \times 10^{-8}$ | 135045 | (3) | $1.49 \times 10^{-7}$ |
| | | $10^{-7}$ | 46277 | (3) | 11042 | (2) | $6.81 \times 10^{-8}$ | 135070 | (3) | $4.69 \times 10^{-8}$ |
| | | $10^{-8}$ | 56658 | (23) | 11052 | (2) | $6.80 \times 10^{-8}$ | 135081 | (3) | $1.33 \times 10^{-9}$ |
| RK5(4)10$_F$[3S*$_+$] | $(0.45, -0.13, 0.00)$ | $10^{-2}$ | 61775 | (1594) | 14420 | (380) | $5.93 \times 10^{-7}$ | 196710 | (3687) | $6.49 \times 10^{-3}$ |
| | | $10^{-3}$ | 51039 | (412) | 14149 | (293) | $4.37 \times 10^{-7}$ | 137587 | (166) | $7.79 \times 10^{-5}$ |
| | | $10^{-4}$ | 46204 | (4) | 11042 | (3) | $1.10 \times 10^{-5}$ | 135129 | (7) | $3.47 \times 10^{-7}$ |
| | | $10^{-5}$ | 46240 | (4) | 11045 | (2) | $3.27 \times 10^{-7}$ | 135079 | (4) | $3.23 \times 10^{-9}$ |
| | | $10^{-6}$ | 46231 | (4) | 11034 | (1) | $6.80 \times 10^{-8}$ | 135081 | (3) | $1.30 \times 10^{-9}$ |
| | | $10^{-7}$ | 46322 | (3) | 11055 | (2) | $6.80 \times 10^{-8}$ | 135084 | (3) | $1.13 \times 10^{-8}$ |
| | | $10^{-8}$ | 54978 | (7) | 11044 | (1) | $6.80 \times 10^{-8}$ | 135096 | (3) | $1.31 \times 10^{-9}$ |

## 3 Detailed results for the viscous shock

Here, we provide detailed performance characteristics of the numerical methods for numerical studies of the viscous shock described in Section 7.1 of the manuscript.

Table 18: Number of function evaluations (#FE), rejected steps (#R), and $L^2$ error of the density for the viscous shock (7.2) using polynomials of degree $p$.

| | | | $p = 2$ | | | $p = 4$ | | |
|---|---|---|---|---|---|---|---|---|
| Scheme | $\beta$ | `tol` | #FE | #R | Error | #FE | #R | Error |
| BS3(2)3$_F$ | $(0.60, -0.20, 0.00)$ | $10^{-2}$ | 689 | (36) | $2.26 \times 10^{-2}$ | 4461 | (249) | $1.64 \times 10^{-2}$ |
| | | $10^{-3}$ | 612 | (1) | $3.77 \times 10^{-3}$ | 3826 | (5) | $2.43 \times 10^{-4}$ |
| | | $10^{-4}$ | 615 | (0) | $3.76 \times 10^{-3}$ | 3842 | (5) | $5.41 \times 10^{-5}$ |
| | | $10^{-5}$ | 615 | (1) | $3.76 \times 10^{-3}$ | 3842 | (3) | $5.42 \times 10^{-5}$ |
| | | $10^{-6}$ | 633 | (0) | $3.76 \times 10^{-3}$ | 3841 | (2) | $5.42 \times 10^{-5}$ |
| | | $10^{-8}$ | 976 | (1) | $3.76 \times 10^{-3}$ | 3838 | (1) | $5.42 \times 10^{-5}$ |
| SSP3(2)4[3S*$_+$] | $(0.55, -0.27, 0.05)$ | $10^{-2}$ | 460 | (16) | $8.37 \times 10^{-3}$ | 2930 | (108) | $1.09 \times 10^{-2}$ |
| | | $10^{-3}$ | 406 | (3) | $3.76 \times 10^{-3}$ | 2488 | (5) | $6.35 \times 10^{-5}$ |
| | | $10^{-4}$ | 410 | (3) | $3.76 \times 10^{-3}$ | 2502 | (4) | $5.42 \times 10^{-5}$ |
| | | $10^{-5}$ | 450 | (1) | $3.76 \times 10^{-3}$ | 2502 | (3) | $5.42 \times 10^{-5}$ |
| | | $10^{-6}$ | 830 | (1) | $3.76 \times 10^{-3}$ | 2518 | (1) | $5.42 \times 10^{-5}$ |
| | | $10^{-8}$ | 2034 | (2) | $3.76 \times 10^{-3}$ | 3626 | (2) | $5.42 \times 10^{-5}$ |
| KCL4(3)5[3R$_+$]C | $(0.41, -0.28, 0.08)$ | $10^{-2}$ | 677 | (19) | $4.84 \times 10^{-3}$ | 4446 | (128) | $7.99 \times 10^{-3}$ |
| | | $10^{-3}$ | 750 | (18) | $1.20 \times 10^{-2}$ | 4003 | (90) | $5.19 \times 10^{-3}$ |
| | | $10^{-4}$ | 537 | (3) | $3.76 \times 10^{-3}$ | 3356 | (28) | $5.82 \times 10^{-5}$ |
| | | $10^{-5}$ | 552 | (2) | $3.76 \times 10^{-3}$ | 3342 | (29) | $5.42 \times 10^{-5}$ |
| | | $10^{-6}$ | 677 | (2) | $3.76 \times 10^{-3}$ | 3447 | (3) | $5.42 \times 10^{-5}$ |
| | | $10^{-8}$ | 1177 | (2) | $3.76 \times 10^{-3}$ | 3542 | (3) | $5.42 \times 10^{-5}$ |
| RK3(2)5$_F$[3S*$_+$] | $(0.70, -0.23, 0.00)$ | $10^{-2}$ | 760 | (44) | $4.85 \times 10^{-3}$ | 4908 | (292) | $3.69 \times 10^{-3}$ |
| | | $10^{-3}$ | 529 | (1) | $3.77 \times 10^{-3}$ | 3257 | (2) | $1.30 \times 10^{-4}$ |
| | | $10^{-4}$ | 523 | (0) | $3.76 \times 10^{-3}$ | 3265 | (2) | $5.41 \times 10^{-5}$ |
| | | $10^{-5}$ | 533 | (0) | $3.76 \times 10^{-3}$ | 3270 | (2) | $5.42 \times 10^{-5}$ |
| | | $10^{-6}$ | 658 | (0) | $3.76 \times 10^{-3}$ | 3269 | (1) | $5.42 \times 10^{-5}$ |
| | | $10^{-8}$ | 1388 | (0) | $3.76 \times 10^{-3}$ | 3429 | (1) | $5.42 \times 10^{-5}$ |
| RK4(3)9[3S*$_+$] | $(0.25, -0.12, 0.00)$ | $10^{-2}$ | 711 | (14) | $3.80 \times 10^{-3}$ | 3979 | (83) | $5.45 \times 10^{-5}$ |
| | | $10^{-3}$ | 684 | (10) | $3.76 \times 10^{-3}$ | 4000 | (69) | $6.63 \times 10^{-5}$ |
| | | $10^{-4}$ | 728 | (8) | $3.76 \times 10^{-3}$ | 4084 | (52) | $5.50 \times 10^{-5}$ |
| | | $10^{-5}$ | 542 | (0) | $3.76 \times 10^{-3}$ | 3403 | (7) | $5.47 \times 10^{-5}$ |
| | | $10^{-6}$ | 659 | (0) | $3.76 \times 10^{-3}$ | 3098 | (1) | $5.42 \times 10^{-5}$ |
| | | $10^{-8}$ | 1190 | (0) | $3.76 \times 10^{-3}$ | 3188 | (1) | $5.42 \times 10^{-5}$ |
| RK5(4)10$_F$[3S*$_+$] | $(0.45, -0.13, 0.00)$ | $10^{-2}$ | 787 | (17) | $3.77 \times 10^{-3}$ | 4671 | (105) | $6.25 \times 10^{-5}$ |
| | | $10^{-3}$ | 662 | (2) | $3.77 \times 10^{-3}$ | 4057 | (4) | $1.51 \times 10^{-4}$ |
| | | $10^{-4}$ | 644 | (1) | $3.76 \times 10^{-3}$ | 3930 | (3) | $5.41 \times 10^{-5}$ |
| | | $10^{-5}$ | 643 | (0) | $3.76 \times 10^{-3}$ | 3931 | (3) | $5.42 \times 10^{-5}$ |
| | | $10^{-6}$ | 777 | (4) | $3.76 \times 10^{-3}$ | 3942 | (2) | $5.42 \times 10^{-5}$ |
| | | $10^{-8}$ | 994 | (1) | $3.76 \times 10^{-3}$ | 4359 | (26) | $5.42 \times 10^{-5}$ |

## References


[37] C. A. Kennedy, M. H. Carpenter, and R. M. Lewis. "Low-storage, explicit Runge-Kutta schemes for the compressible Navier-Stokes equations". In: *Applied Numerical Mathematics* 35.3 (2000), pp. 177–219. DOI: 10.1016/S0168-9274(99)00141-5.
